# Supplementary material for: Shift identification in time varying regression quantiles
Source: arXiv:2011.06333 source file (2021-12-24)
Supplement: Supplementary file 1 [file supplement.pdf]

# Supplementary material to “Comparing time varying regression quantiles under shift invariance”

Subhra Sankar Dhar

IIT Kanpur

Department of Mathematics & Statistics

Kanpur 208016, India

email: subhra@iitk.ac.in

Weichi Wu

Center for Statistical Science

Department of Industrial Engineering

Tsinghua University 100084 Beijing, China

email: wuweichi@mail.tsinghua.edu.cn

## Abstract

This supplementary material contains a sketch of the proofs as well as all the detailed proofs for Theorem 3.1, Theorem 3.2 and [Theorem 5.1](#) in the main article, proof of proposition 2.1 and a remark D.1 on the parameter  $\eta$ . [Moreover, the simulation results for mutually dependent data sets are also available here.](#)

## A Sketch of the Proofs of Theorems 3.1 and 3.2

The properties of the estimators  $\hat{a}$  and  $\hat{b}$  follow from the stochastic expansion of the deviation of the local linear quantile estimator  $\hat{m}_s(t) - m_s(t)$ , (cf. Proposition 1 of Wu and Zhou (2017)) as well as the monotonicity of functions  $\mu_s$ ,  $s = 1$  and  $2$ . The proof of Theorem 3.1 [has](#) two steps. The first step is to expand the deviation of the test statistics under null and local alternatives, and approximate it by certain Gaussian processes using the extended argument of proof of Theorem 4.1 of Dette and Wu (2019). Notice that in our case, we

consider two samples as well as the local linear quantile regression. The second step is to use Theorem 2.1 of de Jong (1987) to figure out the asymptotic behavior of a quadratic Gaussian integrals via tedious calculations. Based on Step 1 of the proof of Theorem 3.1 and using the approximation formula in Proposition 1 of Sun and Loader (1994), we derive the proof of Theorem 3.2, which obtains the simultaneous confidence band. Intensive calculations are provided in our proof to determine the parameters in the approximation formula of Sun and Loader (1994).

## B Proofs of Theorem 3.1 and 3.2.

### B.1 Proof of Theorem 3.1

*Proof.* Write

$$\tilde{T}_{n_1, n_2} = \int_{\mathbb{R}} (\hat{g}_1(t) - \hat{g}_2(t))^2 w(t) dt, \text{ where } w(t) = \mathbf{1}(a + \eta \leq t \leq b - \eta). \quad (\text{B.2})$$

In the following, we shall prove that, under conditions of Theorem 3.1,

$$n_1 b_{n,1}^{5/2} \tilde{T}_{n_1, n_2} - b_{n,1}^{-1/2} (\check{B}_1 + \gamma_0 \gamma_1^3 \check{B}_2) - \int_{\mathbb{R}} \kappa^2(t) w(t) dt \Rightarrow N(0, V_T), \quad (\text{B.3})$$

$$n_1 b_{n,1}^{5/2} (\tilde{T}_{n_1, n_2} - T_{n_1, n_2}) = o_p(1). \quad (\text{B.4})$$

**Proof of (B.3):**

Define  $g_s(t) = \frac{1}{N h_s} \sum_{i=1}^N H\left(\frac{m_s(\frac{i}{N}) - t}{h_s}\right)$ . Then we have the following decomposition:

$$\tilde{T}_{n_1, n_2} = \int_{\mathbb{R}} (J_1(t) - J_2(t) + J_3(t))^2 w(t) dt, \quad (\text{B.5})$$

$$J_s(t) = \hat{g}_s(t) - g_s(t), s = 1 \text{ and } 2, J_3(t) = g_1(t) - g_2(t). \quad (\text{B.6})$$

Using the similar argument of page 471 of Dette et al. (2006), we have

$$\begin{aligned} J_3(t) &= (m_1^{-1})'(t) - (m_2^{-1})'(t) + O\left(h_1 + h_2 + \frac{1}{Nh_1} + \frac{1}{Nh_2}\right) \\ &= \rho_n \kappa(t) + O\left(h_1 + h_2 + \frac{1}{Nh_1} + \frac{1}{Nh_2}\right). \end{aligned} \quad (\text{B.7})$$

Next, by Taylor series expansion, we have that for  $s = 1$  and  $2$ , the following decomposition holds:

$$J_s(t) = J_{s,1}(t) + J_{s,2}(t), \quad (\text{B.8})$$

where

$$\begin{aligned} J_{s,1}(t) &= \frac{1}{Nh_s^2} \sum_{i=1}^N H' \left( \frac{m_s(i/N) - t}{h_s} \right) (\hat{m}_s(i/N) - m_s(i/N)), \\ J_{s,2}(t) &= \frac{1}{2Nh_s^3} \sum_{i=1}^N H'' \left( \frac{m_s(i/N) - t + \nu_s^*(\hat{m}_s(i/N) - m_s(i/N))}{h_s} \right) (\hat{m}_s(i/N) - m_s(i/N))^2 \end{aligned}$$

for some  $\nu_s^* \in [-1, 1]$  ( $s = 1$  and  $2$ ). Notice that  $\frac{\log^{4/3} n_s}{\sqrt{(n_s b_{n,s}) h_s}} = o(1)$ , and thus the number of non-zero summands in  $J_{s,2}(t)$  is of order  $O\left(\frac{\log^{4/3} n_s}{\sqrt{(n_s b_{n,s}) h_s}}\right)$  with probability 1. Using Propositions D.1 and D.2, with the same arguments in the proof of Theorem 4.1 in the online supplement of Dette and Wu (2019) for obtaining bound for  $\Delta_{2,N}$  in their paper, we obtain that for  $s = 1$  and  $2$ , and uniformly for  $t \in [a + \eta, b - \eta]$ ,

$$J_{s,2}(t) = O_p \left( \frac{\log^4 n_s}{(n_s b_{n,s})^{3/2} h_s^2} \right). \quad (\text{B.9})$$

Therefore, by applying the assertion of Proposition D.1 to  $J_{s,1}(t)$ , equations (B.7)–(B.9), on a possibly richer probability space, there exists a sequence of i.i.d. standard normal random variables  $(V_{s,i})_{i \in \mathbb{Z}}$ ,  $s = 1$  and  $2$  such that  $\tilde{T}_{n_1, n_2}$  can be written as

$$\tilde{T}_{n_1, n_2} = \int_{\mathbb{R}} [(m_1^{-1})'(t) - (m_2^{-1})'(t) + Z(t) + R(t)]^2 w(t) dt$$

$$= \int_{\mathbb{R}} [\rho_n \kappa(t) + Z(t) + R(t)]^2 w(t) dt, \quad (\text{B.10})$$

where

$$Z(t) = \sum_{s=1}^2 \frac{(-1)^{s-1}}{n_s b_{n,s} N h_s^2} \sum_{i=1}^N \sum_{j=1}^{n_s} M_{\mathbf{c}_s}(i/N) H' \left( \frac{m_s(i/N) - t}{h_s} \right) \bar{K}_{b_{n,s}}(j/n_s - i/N) V_{j,s}, \quad (\text{B.11})$$

$$\text{and } \sup_{t \in [a+\eta, b-\eta]} |R(t)| = O_p(\Omega_n). \quad (\text{B.12})$$

As

$$n_1 b_{n,1}^{5/2} \rho_n^2 \int_{\mathbb{R}} \kappa^2(t) w(t) dt = \int_{\mathbb{R}} \kappa^2(t) w(t) dt, \quad (\text{B.13})$$

to prove (B.3), it is sufficient to show that

$$n_1 b_{n,1}^{5/2} \int_{\mathbb{R}} Z^2(t) w(t) dt - b_{n,1}^{-1/2} (\check{B}_1 + \gamma_0 \gamma_1^3 \check{B}_2) - \int_{\mathbb{R}} \kappa^2(t) w(t) dt \Rightarrow N(0, V_T), \quad (\text{B.14})$$

$$n_1 b_{n,1}^{5/2} \left( \int_{\mathbb{R}} R(t) (R(t) + \rho_n \kappa(t) + Z(t)) w(t) dt + \int_{\mathbb{R}} \rho_n \kappa(t) Z(t) w(t) dt \right) = o_p(1). \quad (\text{B.15})$$

**Proof of (B.14):**

We decompose  $Z(t)$  by  $Z(t) := Z_1(t) - Z_2(t)$ . Here for  $s = 1$  and  $2$ , we have

$$Z_s(t) = \sum_{j=1}^{n_s} W_s(m_s, j, t) V_{j,s}, \text{ where} \quad (\text{B.16})$$

$$W_s(m_s, j, t) = \frac{1}{n_s b_{n,s} N h_s^2} \sum_{i=1}^N M_{\mathbf{c}_s}(i/N) H' \left( \frac{m_s(i/N) - t}{h_s} \right) \bar{K}_{b_{n,s}}(j/n_s - i/N). \quad (\text{B.17})$$

As a result, we have

$$\int_{\mathbb{R}} (Z_1(t) - Z_2(t))^2 w(t) dt = A_1 + A_2 - 2A_{12}, \text{ where} \quad (\text{B.18})$$

$$A_s = \int_{\mathbb{R}} \left( \sum_{j=1}^{n_s} W_s(m_s, j, t) V_{j,s} \right)^2 w(t) dt, \quad s = 1 \text{ and } 2, \quad (\text{B.19})$$

$$A_{12} = \int_{\mathbb{R}} \left( \sum_{j=1}^{n_1} W_1(m_1, j, t) V_{j,1} \right) \left( \sum_{j=1}^{n_2} W_2(m_2, j, t) V_{j,2} \right) w(t) dt. \quad (\text{B.20})$$

We first prove the results for  $A_1$ , and the result for  $A_2$  can be evaluated in a similar way. Notice that  $A_1 = A_{1,a} + A_{1,b}$ , where

$$A_{1,a} = \sum_{j=1}^{n_1} \left[ \int_{\mathbb{R}} W_1^2(m_1, j, t) w(t) dt \right] V_{j,1}^2, \quad (\text{B.21})$$

$$A_{1,b} = 2 \sum_{1 \leq j_1 < j_2 \leq n_1} \left[ \int_{\mathbb{R}} W_1(m_1, j_1, t) W_1(m_1, j_2, t) w(t) dt \right] V_{j_1,1} V_{j_2,1}. \quad (\text{B.22})$$

Now, using the bandwidth condition  $h_s = o(b_{n,s})$ , calculating the Riemann sum with widths of summands  $1/N$  and change of variable  $y = (m_s(u) - t)/h_s$ , a few steps algebraic calculations show that

$$\begin{aligned} W_s(m_s, j, t) &= \frac{1}{n_s b_{n,s} h_s} \int_{\mathbb{R}} M_{\mathbf{c}_s}(m_s^{-1}(t + h_s y)) H'(y) \times \\ &\quad \bar{K}_{b_{n,s}}(j/n_s - m_s^{-1}(t + h_s y)) (m_s^{-1})'(t + h_s y) dy + O(R(j, s, n, t)), \end{aligned} \quad (\text{B.23})$$

where

$$R(j, s, n, t) = \frac{1}{n_s b_{n,s} h_s^2 N} \mathbf{1} \left( \left| \frac{j/n_s - m_s^{-1}(t)}{b_{n,s} + M h_s} \right| \leq 1 \right) \quad (\text{B.24})$$

for a sufficiently large constant  $M$ . Since  $H$  is chosen to be symmetric, we have  $\int_{\mathbb{R}} H'(x) dx = 0$ . Therefore, by Taylor series expansion, for  $t$  with  $w(t) \neq 0$ , it follows that for  $s = 1$  and 2, the leading term of  $W_s(m_s, j, t)$  can be written as  $\tilde{W}_s(m_s, j, t)(1 + O(b_{n,s} + \frac{h_s}{b_{n,s}}))$ , where

$$\tilde{W}_s(m_s, j, t) = \frac{-1}{n_s b_{n,s}^2} M_{\mathbf{c}_s}(m_s^{-1}(t)) \bar{K}' \left( \frac{j/n_s - m_s^{-1}(t)}{b_{n,s}} \right) ((m_s^{-1})'(t))^2 \int_{\mathbb{R}} H'(y) y dy$$

$$= \frac{-1}{n_s b_{n,s}^2} \check{g}_s(t) \bar{K}' \left( \frac{j/n_s - m_s^{-1}(t)}{b_{n,s}} \right). \quad (\text{B.25})$$

Next, by using (B.25), we have

$$\begin{aligned} \mathbb{E}(A_{1,a}) &= \sum_{j=1}^{n_1} \int_{\mathbb{R}} \tilde{W}_1^2(m_1, j, t) w(t) dt (1 + o(1)) \\ &= \frac{1}{n_1 b_{n,1}^3} \left( \int_{\mathbb{R}} H'(y) dy \right)^2 \int_{\mathbb{R}} \bar{K}'^2(x) dx \int_{\mathbb{R}} M_{\mathbf{c}_1}^2(u) (m_1'(u))^{-3} w(m_1(u)) du (1 + o(1)) \\ &= \frac{1}{n_1 b_{n,1}^3} \check{B}_1 (1 + o(1)). \end{aligned} \quad (\text{B.26})$$

On the other hand, the similar calculations show that

$$\text{Var}(A_{1,a}) = \sum_{j=1}^{n_1} \left[ \int_{\mathbb{R}} W_1^2(m_1, j, t) w(t) dt \right]^2 = O\left(\frac{n_1 b_{n,1}^2}{n_1^4 b_{n,1}^8}\right) = O\left(\frac{1}{n_1^3 b_{n,1}^6}\right). \quad (\text{B.27})$$

Then for  $A_{1,b}$ , we have that due to symmetry of the  $\int_{\mathbb{R}} W_1(m_1, j_1, t) W_1(m_1, j_2, t) w(t) dt$  in  $j_1$  and  $j_2$ ,

$$\begin{aligned} \text{Var}(A_{1,b})/2 &= \sum_{j_1=1}^{n_s} \sum_{j_2=1, j_2 \neq j_1}^{n_s} \left[ \int_{\mathbb{R}} W_1(m_1, j_1, t) W_1(m_1, j_2, t) w(t) dt \right]^2 \\ &= \sum_{j_1=1}^{n_s} \sum_{j_2=1, j_2 \neq j_1}^{n_s} \left[ \int_{\mathbb{R}} \tilde{W}_1(m_1, j_1, t) \tilde{W}_1(m_1, j_2, t) w(t) dt \right]^2 (1 + o(1)) \\ &= \frac{1}{n_s^2 b_{n,s}^8} \int_{\mathbb{R}} \int_{\mathbb{R}} \left[ \int_{\mathbb{R}} \check{g}_1^2(t) \bar{K}' \left( \frac{u - m_1^{-1}(t)}{b_{n,1}} \right) \bar{K}' \left( \frac{v - m_1^{-1}(t)}{b_{n,1}} \right) w(t) dt \right]^2 dudv \\ &\quad \times (1 + o(1)). \end{aligned} \quad (\text{B.28})$$

Now, by changing variable, i.e., letting  $\frac{u - m_1^{-1}(t)}{b_{n,1}} = x$ , and using the fact that  $\tilde{g}_1(m_1(u)) =$

$\check{g}_1^2(m_1(u))w(m_1(u))m'_1(u)$ , we have

$$\begin{aligned}
& \text{Var}(A_{1,b})/2 \\
&= \frac{1}{n_1^2 b_{n,1}^6} \int_{\mathbb{R}} \int_{\mathbb{R}} \left[ \int_{\mathbb{R}} \check{g}_1^2(m_1(u)) \bar{K}'(x) \bar{K}'\left(x + \frac{v-u}{b_{n,1}}\right) w(m(u)) m'(u) dx \right]^2 dudv (1 + o(1)) \\
&= \frac{1}{n_1^2 b_{n,1}^6} \int_{\mathbb{R}} \int_{\mathbb{R}} \check{g}_1^2(m_1(u)) \left[ \int_{\mathbb{R}} \bar{K}'(x) \bar{K}'\left(x + \frac{v-u}{b_{n,1}}\right) dx \right]^2 dudv (1 + o(1)) \\
&= \frac{1}{n_1^2 b_{n,1}^5} \int_{\mathbb{R}} \int_{\mathbb{R}} \check{g}_1^2(m_1(u)) (\bar{K}' \star \bar{K}')(y)^2 dudv (1 + o(1)) = \frac{1}{n_1^2 b_{n,1}^5} \check{V}_1 (1 + o(1)). \tag{B.29}
\end{aligned}$$

Combining (B.26) (B.27) and (B.29), it follows that

$$\mathbb{E}(A_{1,a}) = \frac{1}{n_1 b_{n,1}^3} \check{B}_1 (1 + o(1)), \tag{B.30}$$

$$\text{Var}(A_{1,a}) = O\left(\frac{1}{n_1^3 b_{n,1}^6}\right), \tag{B.31}$$

$$\text{Var}(A_{1,b}) = \frac{2}{n_1^2 b_{n,1}^5} \check{V}_1 (1 + o(1)).$$

Similarly,

$$\mathbb{E}(A_{2,a}) = \frac{1}{n_2 b_{n,2}^3} \check{B}_2 (1 + o(1)), \text{Var}(A_{2,a}) = O\left(\frac{1}{n_2^3 b_{n,2}^6}\right), \text{Var}(A_{2,b}) = \frac{2}{n_2^2 b_{n,2}^5} \check{V}_2 (1 + o(1)). \tag{B.32}$$

On the other hand, for  $A_{12}$ , we have

$$\begin{aligned}
\text{Var}(A_{12}) &= \sum_{j_1=1}^{n_1} \sum_{j_2=1}^{n_2} \left[ \int_{\mathbb{R}} W_1(m_1, j_1, t) W_2(m_2, j_2, t) w(t) dt \right]^2 \\
&= \frac{1}{n_1 n_2 b_{n,1}^4 b_{n,2}^4} \int_{\mathbb{R}} \int_{\mathbb{R}} \left[ \int_{\mathbb{R}} \check{g}_1(t) \check{g}_2(t) \bar{K}'\left(\frac{u - m_1^{-1}(t)}{b_{n,1}}\right) \bar{K}'\left(\frac{v - m_2^{-1}(t)}{b_{n,2}}\right) w(t) dt \right]^2 dudv (1 + o(1)), \tag{B.33}
\end{aligned}$$

(B.34)

By change of variable using  $x = (u - m_1^{-1}(t))/b_{n,1}$ , we have that

$$\begin{aligned}
& \int_{\mathbb{R}} \int_{\mathbb{R}} \left[ \int_{\mathbb{R}} \check{g}_1(t) \check{g}_2(t) \bar{K}' \left( \frac{u - m_1^{-1}(t)}{b_{n,1}} \right) \bar{K}' \left( \frac{v - m_2^{-1}(t)}{b_{n,2}} \right) w(t) dt \right]^2 dudv \\
&= b_{n,1}^2 \int_{\mathbb{R}} \int_{\mathbb{R}} \check{g}_{1,2}^2(m_1(u)) \left[ \int_{\mathbb{R}} \bar{K}'(x) \bar{K}' \left( \frac{m'_{21}(u)b_{n,1}x + v - m_{21}(u)}{b_{n,2}} \right) dx \right]^2 dudv (1 + o(1)) \\
&= b_{n,1}^2 b_{n,2} \int_{\mathbb{R}} \int_{\mathbb{R}} \check{g}_{1,2}^2(m_1(u)) \left[ \int_{\mathbb{R}} \bar{K}'(x) \bar{K}' \left( \frac{m'_{21}(u)b_{n,1}x}{b_{n,2}} + y \right) dx \right]^2 dudy (1 + o(1)). \quad (\text{B.35})
\end{aligned}$$

Therefore, we have that

$$I = \frac{\check{V}_{12}(\gamma_1)}{n_1 n_2 b_{n,1}^2 b_{n,2}^3} (1 + o(1)) \quad (\text{B.36})$$

Notice that  $A_{1,b}$ ,  $A_{2,b}$ ,  $A_{12}$  are mutually uncorrelated. Using this fact, bandwidth conditions and (B.18), (B.30), (B.32) and (B.36), equation (B.14) follows from Theorem 2.1 of de Jong (1987) and tedious calculations.

**Proof of (B.15):** By (B.16), (B.17), (B.23)-(B.25), we obtain for  $s = 1, 2$

$$\sup_{t \in [0,1]} |Z_s(t)| = \frac{\sqrt{\log n_s}}{\sqrt{n_s b_{n,s} b_{n,s}}}, \quad (\text{B.37})$$

which together with bandwidth conditions yields (B.15). Hence (B.3) holds.

**Proof of Theorem 3.1 (conclusion part):** By the proof of (B.3) and the bandwidth conditions, it suffices to show that

$$n_1 b_{n,1}^{5/2} \int_{\mathbb{R}} (Z(t))^2 (\hat{w}(t) - w(t)) dt = o_p(1). \quad (\text{B.38})$$

Meanwhile, assertion in (B.38) follows from (B.37), Proposition D.3 and bandwidth conditions. Now, by (B.3) and (B.4), Theorem 3.1 follows.  $\square$

## B.2 Proof of Theorem 3.2

*Proof.* We prove the theorem in two steps.

Step 1: Recall  $Z(t)$  defined in (B.11) in the proof of Theorem 3.1 . We first evaluate  $\mathbb{E}(Z^2(t))$ ,  $\mathbb{E}(Z'^2(t))$  and  $\mathbb{E}(Z(t)Z'(t))$ . Since  $h_s = o(b_{n,s})$ , uniformly for  $t \in [a + \eta, b - \eta]$ , we have

$$\begin{aligned}
\mathbb{E}(Z^2(t)) &= \sum_{s=1}^2 \frac{1}{(n_s b_{n,s} N h_s^2)^2} \sum_{j=1}^{n_s} \left( \sum_{i=1}^N M_{\mathbf{c}_s}(i/N) H' \left( \frac{m_s(i/N) - t}{h_s} \right) \bar{K}_{b_{n,s}}(j/n_s - i/N) \right)^2 \\
&= \sum_{s=1}^2 \frac{1}{(n_s b_{n,s} h_s^2)^2} \sum_{j=1}^{n_s} \left( \int_{\mathbb{R}} M_{\mathbf{c}_s}(u) H' \left( \frac{m_s(u) - t}{h_s} \right) \bar{K}_{b_{n,s}}(j/n_s - u) du + O \left( \frac{\mathbf{1}(|j/n_s - t| \leq \bar{M} b_{n,s})}{N} \right) \right)^2 \\
&= \sum_{s=1}^2 \frac{1}{n_s (b_{n,s} h_s^2)^2} \int_{\mathbb{R}} \left( \int_{\mathbb{R}} M_{\mathbf{c}_s}(u) H' \left( \frac{m_s(u) - t}{h_s} \right) \bar{K}_{b_{n,s}}(v - u) du \right)^2 dv + O \left( \frac{1}{n_s^2 b_{n,s}^2 h_s^2} + \frac{1}{n_s N b_{n,s}^2 h_s^2} \right) \\
&= \sum_{s=1}^2 \frac{M_{\mathbf{c}_s}^2(m_s^{-1}(t))}{n_s (b_{n,s} h_s)^2 (m'_s(m_s^{-1}(t)))^2} \int_{\mathbb{R}} \left( \int_{\mathbb{R}} H'(x) \bar{K}_{b_{n,s}}(v - m_s^{-1}(t + x h_s)) dx \right)^2 dv + O \left( \frac{1}{n_s b_{n,s} h_s} \right) \\
&= \sum_{s=1}^2 \frac{M_{\mathbf{c}_s}^2(m_s^{-1}(t)) (m_s^{-1})'^2(t)}{n_s b_{n,s}^3 (m'_s(m_s^{-1}(t)))^2} \int_{\mathbb{R}} \bar{K}'^2(y) dy \left( \int_{\mathbb{R}} H'(x) x dx \right)^2 \left( 1 + O \left( \frac{h_s}{b_{n,s}} \right) \right) + O \left( \frac{1}{n_s b_{n,s} h_s} \right).
\end{aligned}$$

Next, we have

$$\begin{aligned}
\mathbb{E}(Z'^2(t)) &= \sum_{s=1}^2 \frac{1}{(n_s b_{n,s} N h_s^3)^2} \sum_{j=1}^{n_s} \left( \sum_{i=1}^N M_{\mathbf{c}_s}(i/N) H'' \left( \frac{m_s(i/N) - t}{h_s} \right) \bar{K}_{b_{n,s}}(j/n_s - i/N) \right)^2 \\
&= \sum_{s=1}^2 \frac{1}{(n_s b_{n,s} h_s^3)^2} \sum_{j=1}^{n_s} \left( \int_{\mathbb{R}} M_{\mathbf{c}_s}(u) H'' \left( \frac{m_s(u) - t}{h_s} \right) \bar{K}_{b_{n,s}}(j/n_s - u) du \left( 1 + O \left( \frac{1}{N h_s} \right) \right) \right)^2 \\
&= \sum_{s=1}^2 \frac{1}{n_s (b_{n,s} h_s^3)^2} \int_{\mathbb{R}} \left( \int_{\mathbb{R}} M_{\mathbf{c}_s}(u) H'' \left( \frac{m_s(u) - t}{h_s} \right) \bar{K}_{b_{n,s}}(v - u) du \right)^2 dv \left( 1 + O \left( \frac{1}{N h_s} \right) \right)
\end{aligned}$$

$$\begin{aligned}
& + O\left(\frac{1}{n_s^2 b_{n,s}^2 h_s^4}\right) \\
& = \sum_{s=1}^2 \frac{M_{\mathbf{c}_s}^2(m_s^{-1}(t))}{n_s(b_{n,s}h_s^2)^2(m'_s(m_s^{-1}(t)))^2} \int_{\mathbb{R}} \left( \int_{\mathbb{R}} H''(x) \bar{K}_{b_{n,s}}(v - m_s^{-1}(t + xh_s)) dx \right)^2 dv \left( 1 + O\left(\frac{1}{Nh_s}\right) \right) \\
& \quad + O\left(\frac{1}{n_s b_{n,s} h_s^3}\right) \\
& = \sum_{s=1}^2 \frac{M_{\mathbf{c}_s}^2(m_s^{-1}(t))}{n_s b_{n,s} h_s^4 (m'_s(m_s^{-1}(t)))^2} \int_{\mathbb{R}} \bar{K}^2(y) dy \left( \int_{\mathbb{R}} H''(x) dx \right)^2 \left( 1 + O\left(\frac{1}{Nh_s} + \frac{h_s}{b_{n,s}}\right) \right) + O\left(\frac{1}{n_s b_{n,s} h_s^3}\right).
\end{aligned}$$

Finally, by the symmetry of  $K$  and  $H$ , we have

$$\begin{aligned}
& \mathbb{E}(Z(t)Z'(t)) \\
& = \sum_{s=1}^2 \frac{1}{(n_s b_{n,s} N h_s^2)^2 h_s} \sum_{j=1}^{n_s} \left( \sum_{i=1}^N M_{\mathbf{c}_s}(i/N) H' \left( \frac{m_s(i/N) - t}{h_s} \right) \bar{K}_{b_{n,s}}(j/n_s - i/N) \right) \\
& \quad \times \left( \sum_{i=1}^N M_{\mathbf{c}_s}(i/N) H'' \left( \frac{m_s(i/N) - t}{h_s} \right) \bar{K}_{b_{n,s}}(j/n_s - i/N) \right) \\
& = \sum_{s=1}^2 \frac{1}{(n_s b_{n,s} h_s^2)^2 h_s} \sum_{j=1}^{n_s} \left( \int_{\mathbb{R}} M_{\mathbf{c}_s}(u) H' \left( \frac{m_s(u) - t}{h_s} \right) \bar{K}_{b_{n,s}}(j/n_s - u) du + O\left(\frac{\mathbf{1}(|j/n_s - t| \leq \bar{M}b_{n,s})}{N}\right) \right) \\
& \quad \left( \int_{\mathbb{R}} M_{\mathbf{c}_s}(u) H'' \left( \frac{m_s(u) - t}{h_s} \right) \bar{K}_{b_{n,s}}(j/n_s - u) du + O\left(\frac{\mathbf{1}(|j/n_s - t| \leq \bar{M}b_{n,s})}{N}\right) \right) \\
& = \sum_{s=1}^2 \frac{1}{n_s(b_{n,s}h_s^2)^2 h_s} \int_{\mathbb{R}} \left( \int_{\mathbb{R}} M_{\mathbf{c}_s}(u) H' \left( \frac{m_s(u) - t}{h_s} \right) \bar{K}_{b_{n,s}}(v - u) du \right) \\
& \quad \left( \int_{\mathbb{R}} M_{\mathbf{c}_s}(u) H'' \left( \frac{m_s(u) - t}{h_s} \right) \bar{K}_{b_{n,s}}(v - u) du \right) dv + O\left(\frac{1}{n_s^2 b_{n,s}^2 h_s^3} + \frac{1}{n_s N b_{n,s} h_s^4}\right) \\
& = \sum_{s=1}^2 \frac{M_{\mathbf{c}_s}^2(m_s^{-1}(t))}{n_s(b_{n,s}h_s^2)^2 h_s m'_s(m_s^{-1}(t))} \int_{\mathbb{R}} \left( \int_{\mathbb{R}} H'(x) \bar{K}_{b_{n,s}}(v - m_s^{-1}(t + xh_s)) dx \right) \\
& \quad \left( \int_{\mathbb{R}} H''(x) \bar{K}_{b_{n,s}}(v - m_s^{-1}(t + xh_s)) dx \right) dv + O\left(\frac{1}{n b_{n,s} h_s^2}\right)
\end{aligned}$$

$$= O\left(\frac{h_s + (h_s/b_{n,s})^2}{n_s b_{n,s} h_s^3}\right).$$

Step 2: We use Proposition 1 of Sun and Loader (1994) to evaluate the maximum deviation of  $Z(t)$ . For any two  $p$ -dimensional vectors  $\mathbf{u} = (u_1, \dots, u_p)^\top$  and  $\mathbf{v} = (v_1, \dots, v_p)^\top$ , write  $\langle \mathbf{u}, \mathbf{v} \rangle = \sum_{i=1}^p u_i v_i$ , and  $\|\mathbf{u}\|_E = \langle \mathbf{u}, \mathbf{u} \rangle^{1/2}$ . Define

$$T_{j,s}(t) = w_s(m_s, j, t), s = 1 \text{ and } 2, 1 \leq j \leq n_s, \quad (\text{B.39})$$

$$\mathbf{T}(x) = \left(T_{1,1}(x), \dots, T_{n_1,1}(x), T_{1,2}(x), \dots, T_{n_2,2}(x)\right)^\top, \quad (\text{B.40})$$

and  $\mathbf{V} = (V_1, \dots, V_{n_1}, V_{n_1+1}, \dots, V_{n_1+n_2})^\top$ , where  $\{V_i\}_{i=1}^{n_1+n_2}$  is a i.i.d. sequence of standard normal random variables. Then, for any  $0 < a < b < 1$  and  $\eta > 0$ ,  $\sup_{t \in [a,b]} |Z(t)|$  has the same distribution as  $\sup_{t \in [a+\eta, b-\eta]} |\langle \mathbf{T}(t), \mathbf{V} \rangle|$ . Therefore, by Proposition 1 of Sun and Loader (1994), we have that

$$\lim_{c \rightarrow \infty} \mathbb{P}\left(\sup_{t \in [a,b]} |\langle \frac{\mathbf{T}(t)}{\|\mathbf{T}(t)\|_E}, \mathbf{V} \rangle| \geq c\right) = \frac{\kappa_0(a+\eta, b-\eta)}{\pi} \exp\left(-\frac{c^2}{2}\right) + 2(1 - \phi(c)) + o(\exp(-c^2/2)), \quad (\text{B.41})$$

where  $\kappa_0(a+\eta, b-\eta) = \int_{a+\eta}^{b-\eta} \left\| \frac{\partial}{\partial x} \left( \frac{\mathbf{T}(x)}{\|\mathbf{T}(x)\|_E} \right) \right\|_E dx$ . Notice that

$$\|\mathbf{T}(x)\|_E = \|Z(x)\|, \quad \left\| \frac{\partial \mathbf{T}(x)}{\partial x} \right\|_E = \left\| \frac{\partial}{\partial x} Z(x) \right\|, \quad (\text{B.42})$$

$$\frac{\partial}{\partial x} \|\mathbf{T}(x)\|_E = \frac{\langle \mathbf{T}(x), \frac{\partial}{\partial x} \mathbf{T}(x) \rangle}{\|\mathbf{T}(x)\|_E} = \frac{\mathbb{E}(Z(t)Z'(t))}{\|Z(t)\|}, \text{ and} \quad (\text{B.43})$$

$$\left\| \frac{\partial}{\partial x} \left( \frac{\mathbf{T}(x)}{\|\mathbf{T}(x)\|_E} \right) \right\|_E = \left\| \frac{\frac{\partial}{\partial x} \mathbf{T}(x) \|\mathbf{T}(x)\|_E - \frac{\partial}{\partial x} \|\mathbf{T}(x)\|_E \mathbf{T}(x)}{\|\mathbf{T}(x)\|_E^2} \right\|_E. \quad (\text{B.44})$$

By using (B.42)–(B.44) and the results of  $\mathbb{E}(Z^2(t))$ ,  $\mathbb{E}(Z'^2(t))$  and  $\mathbb{E}(Z(t)Z'(t))$  from Step

1, we have that

$$\left\| \frac{\partial}{\partial x} \left( \frac{\mathbf{T}(x)}{\|\mathbf{T}(x)\|_E} \right) \right\|_E = \frac{b_{n,1}}{h_1^2} \sqrt{\frac{K_2(t)}{K_1(t)}} (1 + o(1)). \quad (\text{B.45})$$

Furthermore, by (D.54), we have

$$\lim_{n_1 \rightarrow \infty} \mathbb{P} \left( \max(|\hat{a} - m_1(0)|, |\hat{b} - m_1(1 - m_2^{-1}(m_1(0)))|) \leq \eta/2 \right) = 1. \quad (\text{B.46})$$

Therefore,

$$\begin{aligned} & \mathbb{P} \left( \sup_{t \in [\hat{m}_1(0) + 3\eta/2, \hat{m}_1(1 - m_2^{-1}(m_1(0))) - 3\eta/2]} \left| \left\langle \frac{\mathbf{T}(t)}{\|\mathbf{T}(t)\|_E}, \mathbf{V} \right\rangle \right| \geq c \right) \\ & \leq \mathbb{P} \left( \sup_{t \in [\hat{a} + \eta, \hat{b} - \eta]} \left| \left\langle \frac{\mathbf{T}(t)}{\|\mathbf{T}(t)\|_E}, \mathbf{V} \right\rangle \right| \geq c \right) \\ & \leq \mathbb{P} \left( \sup_{t \in [\hat{m}_1(0) + \eta/2, \hat{m}_1(1 - m_2^{-1}(m_1(0))) - \eta/2]} \left| \left\langle \frac{\mathbf{T}(t)}{\|\mathbf{T}(t)\|_E}, \mathbf{V} \right\rangle \right| \geq c \right). \end{aligned} \quad (\text{B.47})$$

As a consequence, by (B.45), (B.41) and (B.47), and the fact that  $\eta = o(1)$ , the theorem follows when choosing  $c = \sqrt{-2 \log(\pi\alpha/\kappa_0)}$ .

## C Proof of Proposition 2.1

In this subsection we prove Proposition 2.1 in the main article, which enables us to test the null hypothesis  $H_0$  in (1.3) via investigating  $(m_1^{-1}(u))' - (m_2^{-1}(u))'$ .

**Proof of Proposition 2.1:** We extend the proof of Lemma 2.1 in Dette et al. (2021). We shall show (1.3) is equivalent to

$$(m_2^{-1}(u) - m_1^{-1}(u))' = 0 \quad (\text{C.48})$$

for  $m_1(0) < u < m_1(1 - d)$ .

If  $m_1(t) = m_2(t + d)$  for  $0 < t < 1 - d$  for some unknown  $d$ , and  $m_1(t)$  and  $m_2(t)$  are

monotonically increasing for  $0 < t < 1 - d$ , one then can write  $u = m_1(t) = m_2(t + d)$  for  $m_1(0) < u < m_1(1 - d)$ , which implies that  $t = m^{-1}(u)$  and  $t + d = m_2^{-1}(u)$ . Therefore,

$$(m_2^{-1}(u) - m_1^{-1}(u)) = d$$

for  $m_1(0) < u < m_1(1 - d)$ . Since  $d$  is a constant, we have proven that (1.3) implies (C.48).

On the other hand, by (C.48), one can see that for any  $t \in (m_1(0), m_1(1 - d))$ ,

$$\int_{m_1(0)}^t (m_1^{-1}(u))' du = \int_{m_1(0)}^t (m_2^{-1}(u))' du. \quad (\text{C.49})$$

As a result, we have  $m_1^{-1}(t) = m_2^{-1}(t) - m_2^{-1}(m_1(0))$ , and  $d = m_2^{-1}(m_1(0))$ . Therefore, by rearranging the equation and taking  $m_2'$  on both sides of it, one can conclude that

$$t = m_2(m_1^{-1}(t) + m_2^{-1}(m_1(0))) = m_1(m_1^{-1}(t)) \quad (\text{C.50})$$

for  $0 < m_1^{-1}(t) < 1 - d$ , which finishes the proof by setting  $u = m_1^{-1}(t)$ .  $\square$

## D Technical propositions for proving Theorems 3.1 and 3.2.

In the section, we discuss three propositions that are needed for the proof of Theorems 3.1 and 3.2. We first have the following result related to uniform approximation of  $\hat{m}_s(t) - m_s(t)$  through a Gaussian process. The proof of this proposition is based on a Bahadur Representation of  $\hat{m}_s(t) - m_s(t)$ .

**Proposition D.1** *Assume conditions (A1)-(A8) and (B3). Then on a possibly richer probability space, there exist an i.i.d. sequence of standard normal random variables  $(V_{i,1})_{i \in \mathbb{Z}}$  and  $(V_{i,2})_{i \in \mathbb{Z}}$ , such that for  $s = 1$  and  $2$ ,*

$$\sup_{t \in \mathcal{T}_{n,s}} \left| \hat{m}_s(t) - m_s(t) - \frac{M_{\mathbf{c}_s}(t) \sum_{i=1}^{n_s} V_{i,s} \bar{K}_{b_{n,s}}(i/n_s - t)}{nb_{n,s}} \right| = O_p(\Theta_{n,s}), \quad (\text{D.51})$$

where  $\Theta_{n,s}$  is defined in the main article above condition (B1).

*Proof.* The proposition follows immediately from equation (59) of the supplemental material of Wu and Zhou (2017).  $\square$

Therefore we have the following proposition regarding the magnitude of  $|\hat{m}_s(t) - m_s(t)|$ .

**Proposition D.2** *Along with the conditions of Proposition D.1, assume that  $\pi_{n,s} = o(\sqrt{\log n_s})$ ,  $n_s b_{n,s}^2 \log^2 n_s \rightarrow \infty$  for  $s = 1$  and 2. Then, we have that for  $s = 1$  and 2,*

$$\sup_{t \in \mathcal{T}_{n,s}} |\hat{m}_s(t) - m_s(t)| = O_p \left( \frac{\sqrt{\log n_s}}{\sqrt{n_s b_{n,s}}} \right). \quad (\text{D.52})$$

*Proof.* It follows from Lemma 1 of Zhou and Wu (2010) that

$$\sup_{t \in \mathcal{T}_{n,s}} \left| \frac{\sum_{i=1}^{n_s} V_{i,s} \bar{K}_{b_{n,s}}(i/n_s - t)}{n_s b_{n,s}} \right| = O_p \left( \frac{\sqrt{\log n}}{\sqrt{n_s b_{n,s}}} \right). \quad (\text{D.53})$$

Then the assertion of this proposition follows from Proposition D.1.  $\square$

The following proposition provides the convergence rate of  $\hat{a}$  and  $\hat{b}$  under the null and the local alternatives.

**Proposition D.3** *Under the conditions of Proposition D.1, assuming (B1), (B2) and  $\eta = o(1)$ ,  $\eta^{-1} = O(\log(n_1 + n_2))$ . Then if  $(m_1^{-1})'(t) - (m_2^{-1})'(t) = \rho_{n_1, n_2} \kappa(t)$  for some non-zero bounded function  $\kappa(t)$  and  $\rho_{n_1, n_2} = o(\eta)$ , we have that*

$$i) \max(|\hat{a} - m_1(0)|, |\hat{b} - m_1(1 - m_2^{-1}(m_1(0)))|) = O_p \left( \sum_{s=1}^2 \frac{\sqrt{\log n_s}}{\sqrt{n_s b_{n,s} b_{n,s}}} + \rho_{n_1, n_2} \right). \quad (\text{D.54})$$

Notice that under null, the LHS of (D.54) will be reduced to  $\max(|\hat{a} - a|, |\hat{b} - b|)$ . Moreover,

$$ii) \lim_{n_1 \rightarrow \infty, n_2 \rightarrow \infty} \mathbb{P}(m_s^{-1}(t) \in (b_n, 1 - b_n), s = 1, 2, \text{ for all } t \in (\hat{a} + c_1 \eta, \hat{b} - c_2 \eta)) = 1. \quad (\text{D.55})$$

for any given positive constant  $c_1, c_2 > 0$ .

**Remark D.1** Note that i) in Proposition D.3 shows that  $\hat{w}(t)$  in (2.9) is consistent under null hypothesis and local alternatives. Further, observe that ii) in Proposition D.3 shows that by introducing  $\eta$ , we avoid bandwidth conditions since ii) excludes regions where  $m_s^{-1}(t)$  ( $s = 1$  and  $2$ ) are close to 0 and 1.

**Proof of Proposition D.3:** Notice that  $(m_2)^{-1}(t) - (m_1')^{-1}(t) = \rho_{n_1, n_2} \kappa(t)$  implies that

$$m_2^{-1}(u) - m_1^{-1}(u) = m_2^{-1}(m_1(0)) + \int_{m_1(0)}^u \rho_{n_1, n_2} \kappa(t) dt. \quad (\text{D.56})$$

Proof of assertion i): By proposition D.2 and (D.56), it is sufficient to show that for  $s = 1$  and  $2$ ,

$$\sup_{u \in [a, b]} |\hat{g}_s(u) - g_s(u)| = O_p \left( \frac{\sqrt{\log n_s}}{\sqrt{(n_s b_{n,s}) b_{n,s}}} \right), \quad (\text{D.57})$$

where  $g_s(t) = \frac{1}{N h_s} \sum_{i=1}^N H \left( \frac{\hat{m}_s(\frac{i}{N}) - t}{h_s} \right)$ . After carefully inspecting the proof of Theorem 3.1, one can find that  $\sup_{t \in [a, b]} |\hat{g}_s(t) - g_s(t)| = O_p \left( \sup_{t \in [a, b]} Z_s(t) \right)$ , where  $Z_s(t)$  is defined in (B.16) in the proof of Theorem 3.1. Then i) of the proposition follows from (B.37) in the proof of Theorem 3.1. The assertion in (ii) follows from condition (B2), (D.56) (with  $u = \hat{m}_1 \left( 1 - \hat{d} \right)$  especially), strict monotonicity of  $m_s$   $s = 1$  and  $2$ , the mean value theorem and the fact that  $b_{n_1} = o(\eta)$ ,  $b_{n_2} = o(\eta)$  and  $\rho_{n_1, n_2} = o(\eta)$ , which can be explained as follows. Note that using (i), with probability tending to 1, we have

$$m_1(0) < \hat{a}_1 + c_1 \eta. \quad (\text{D.58})$$

Now, since  $b_{n_1} = o(\eta)$ , and  $m_1^{-1}$  is differentiable, using mean value theorem with probability tending to 1, we have

$$m_1(b_{n_1}) < \hat{a} + c_1 \eta, \quad (\text{D.59})$$

and hence,  $\lim_{n \rightarrow \infty} \mathbb{P}(b_{n_1} < m_1^{-1}(\hat{a} + c_1 \eta)) = 1$ . Arguing in a similar way, one can establish that  $\lim_{n \rightarrow \infty} \mathbb{P}(1 - b_{n_1} > m_1^{-1}(\hat{b} - c_2 \eta)) = 1$ . Then (ii) holds since the function  $m^{-1}(\cdot)$  is

monotone. □

## E Proof of results of Section 5

In this section, we assume that  $n_1 \geq n_2$ ,  $1 \leq n_1/n_2 \leq M < \infty$  for some large constant  $M$ . Here we stick to the scenario that two series are both collected in the same period, i.e.,  $\tilde{\mathbf{y}}_{i,1}$  is realized at time  $\frac{i}{n_1}$  for  $1 \leq i \leq n_1$ , and  $\tilde{\mathbf{y}}_{i,2}$  is realized at time  $\frac{\lfloor in_1/n_2 \rfloor}{n_1}$  for  $1 \leq i \leq n_2$ .

**Proposition E.1** *Under the conditions of Proposition D.1 with (A7) replaced by (A7'), then on a possibly richer probability space, there exist an i.i.d. sequence of normal  $N\left(0, \begin{pmatrix} 1 & 0 \\ 0 & 1 \end{pmatrix}\right)$  random vectors  $\mathbf{V}_i = (V_{i,1}, V_{i,2})^\top$  such that*

$$\sup_{t \in \mathcal{T}_{n,1} \cap \mathcal{T}_{n,2}} \left| \hat{m}_1(t) - m_1(t) - \frac{\sum_{i=1}^{n_1} (M_{1,1}^c(t)V_{i,1} + M_{1,2}^c(t)V_{i,2})\bar{K}_{b_{n,1}}(i/n_1 - t)}{nb_{n,1}} \right| = O_p(\Theta_{n,1}), \quad (\text{E.60})$$

$$\sup_{t \in \mathcal{T}_{n,1} \cap \mathcal{T}_{n,2}} \left| \hat{m}_2(t) - m_2(t) - \frac{\sum_{i=1}^{n_2} (M_{1,2}^c(t)V_{i',1} + M_{2,2}^c(t)V_{i',2})\bar{K}_{b_{n,2}}(i'/n_1 - t)}{nb_{n,2}} \right| = O_p(\Theta_{n,2}), \quad (\text{E.61})$$

where  $i' = \lfloor in_1/n_2 \rfloor$ .

*Proof.* By Lemma 7 of Wu and Zhou (2017), we have

$$\max_{s=1,2} \sup_{t \in \mathcal{T}_{n,s}} |\tilde{\boldsymbol{\theta}}_{\tau,s,b_{n,s}}(t) - \boldsymbol{\theta}_{\tau,s}(t) - \boldsymbol{\Sigma}_s^{-1}(t) \frac{\sum_{i=1}^{n_s} \psi(e_{i,s})\mathbf{x}_{i,s}\bar{K}_{b_{n,s}}(i/n_s - t)}{nb_{n,s}}| = O_p(\max_{s=1,2} (n_s b_{n,s})^{-1/2} \pi_{n,s}), \quad (\text{E.62})$$

where  $\pi_{n,s}$  is defined in Proposition D.1. By Proposition 3 in Wu and Zhou (2017), for any  $s \times p$  ( $s \leq p$ ) matrix  $\mathbf{C}$ , we have on a possibly richer probability space, there exists an

i.i.d. sequence of normal  $N\left(0, \begin{pmatrix} 1 & 0 \\ 0 & 1 \end{pmatrix}\right)$  random vectors  $\mathbf{V}_i = (V_{i,1}, V_{i,2})^\top$  such that

$$\max_{1 \leq j \leq n_1} \left| \sum_{i=1}^j \mathbf{U}\left(\frac{i}{n_1}, \mathcal{F}_i, \mathcal{G}_i\right) - \sum_{i=1}^j \boldsymbol{\nu}_{\mathbf{C}}(i/n_1) \mathbf{V}_i \right| = O_p(n_1^{1/4} \log n_1) \quad (\text{E.63})$$

with  $\boldsymbol{\nu}_{\mathbf{C}}(t) = (\mathbf{C}\mathbf{V}^2(t)\mathbf{C}^\top)^{1/2}$ . Now, define the index set  $A = \{\lfloor \frac{i}{n_2} n_1 \rfloor, 1 \leq i \leq n_2\}$  and observe that for any bandwidth  $b_n$ , we have

$$\sum_{i=1}^{n_2} \psi(e_{i,2}) \mathbf{x}_{i,2} K_{b_n}(\lfloor i n_1 / n_2 \rfloor / n_1 - t) = \sum_{i=1}^{n_1} \psi(e_{i,1}) \mathbf{x}_{i,1} K_{b_n}(i/n_1 - t) \mathbf{1}(i \in A). \quad (\text{E.64})$$

Let us now consider

$$\Delta_1 = \sup_{t \in \mathcal{T}_{n,1}} \left| \tilde{\boldsymbol{\theta}}_{\tau,1,b_{n,1}}(t) - \boldsymbol{\theta}_{\tau,1}(t) - \boldsymbol{\Sigma}_1^{-1}(t) \frac{\sum_{i=1}^{n_1} \psi(e_{i,1}) \mathbf{x}_{i,1} \bar{K}_{b_{n,1}}(i/n_1 - t)}{n b_{n,1}} \right|, \quad (\text{E.65})$$

$$\Delta_2 = \sup_{t \in \mathcal{T}_{n,2}} \left| \tilde{\boldsymbol{\theta}}_{\tau,2,b_{n,2}}(t) - \boldsymbol{\theta}_{\tau,2}(t) - \boldsymbol{\Sigma}_2^{-1}(t) \frac{\sum_{i=1}^{n_1} \psi(e_{i,1}) \mathbf{x}_{i,1} \bar{K}_{b_{n,2}}(i/n_1 - t) \mathbf{1}(i \in A)}{n b_{n,2}} \right|, \quad (\text{E.66})$$

then (E.62) can be written as

$$\max(\Delta_1, \Delta_2) = O_p(\max_{s=1,2} (n_s b_{n,s})^{-1/2} \pi_{n,s}). \quad (\text{E.67})$$

Use the expression, an application of summation by part formula together with (E.63), we have

$$\sup_{t \in \mathcal{T}_{n,1} \cap \mathcal{T}_{n,2}} \left| \begin{pmatrix} \hat{m}_1(t) - m_1(t) \\ \hat{m}_2(t) - m_2(t) \end{pmatrix} - \sum_{i=1}^{n_1} \mathbf{K}(i, t) \mathbf{M}_{\mathbf{C}}(t) \mathbf{V}_i \right| = O_p(\max_{s=1,2} \Theta_{n,s}), \quad (\text{E.68})$$

where

$$\mathbf{K}(i, t) = \begin{pmatrix} \bar{K}_{b_{n,1}}(i/n_1 - t) / (n b_{n,1}) \\ \bar{K}_{b_{n,2}}(i/n_1 - t) / (n b_{n,2}) \mathbf{1}(i \in A) \end{pmatrix}. \quad (\text{E.69})$$

Straightforward calculation shows that (E.68) implies both the two assertions of the proposition.  $\square$

**Proposition E.2** *Let  $\rho_n = o(1)$ , and assume for  $t \in [a, b]$ ,  $(m_1^{-1} - m_2^{-1})'(t) = \rho_n \kappa(t)$  for some bounded function  $\kappa(t)$ , where  $a = m_1(0) \wedge m_2(0)$  and  $b = m_1(1) \vee m_2(1)$ . Then for any  $u \in [m_1(0) \wedge m_2(0), m_1(1) \vee m_2(1)]$ , we have*

$$m_1^{-1}(u) - m_2^{-1}(u) = -m_2^{-1}(m_1(0)) + O(\rho_n) = m_1^{-1}(m_2(0)) + O(\rho_n). \quad (\text{E.70})$$

*In particular,*

$$t - m_2^{-1}(m_1(t)) = -m_2^{-1}(m_1(0)) + O(\rho_n) = m_1^{-1}(m_2(0)) + O(\rho_n), \quad (\text{E.71})$$

$$m_1^{-1}(m_2(t)) - t = -m_2^{-1}(m_1(0)) + O(\rho_n) = m_1^{-1}(m_2(0)) + O(\rho_n). \quad (\text{E.72})$$

*Proof.* Observe that

$$m_1^{-1}(t) - m_2^{-1}(t) - (0 - m_2^{-1}(m_1(0))) = \int_{m_1(0)}^t (m_1^{-1}(s) - m_2^{-1}(s))' ds, \quad (\text{E.73})$$

$$m_1^{-1}(t) - m_2^{-1}(t) - (m_1^{-1}(m_2(0)) - 0) = \int_{m_2(0)}^t (m_1^{-1}(s) - m_2^{-1}(s))' ds \quad (\text{E.74})$$

Notice that Under  $H_0$   $m_1(0) = m_2(0)$ , so  $m_2^{-1}(m_1(0)) = 0$ , and by the fact that  $(m_1^{-1} - m_2^{-1})'(t) = \rho_n \kappa(t)$ , the proposition follows.  $\square$

To prove the assertion in Theorem 5.1, we shall study the asymptotic behavior of  $T_{n_1, n_2}$  and  $\hat{m}_1^{-1} - \hat{m}_2^{-1}(t)$  under the case that the two time series are correlated. The results are presented and proved in Theorem E.1 and E.2 below, respectively.

Let us first consider the following variables:

$$\check{g}_{uv}(t) = M_{uv}^c(m_u^{-1}(t))((m_u^{-1})'(t))^2 \int_R H'(y) y dy, \quad (\text{E.75})$$

$$(\text{E.76})$$

Define the following quantities with  $r, a, b, c$  functions of  $u$ ,  $a^*, b^* \in \mathbb{R}$ ,

$$\tilde{E}_1 = \int \bar{K}'^2(u) du \int \check{g}_{11}^2(m_1(x)) w(m_1(x)) m_1'(x) dx, \quad (\text{E.77})$$

$$\tilde{C}_1 = \int (\bar{K}' \star \bar{K}'(z))^2 dz \int (\check{g}_{11}^2(m_1(x))w(m_1(x))m_1'(x))^2 dx \quad (\text{E.78})$$

$$\tilde{E}_2 = \int \bar{K}'^2(u) du \int \check{g}_{21}^2(m_2(x))w(m_2(x))m_2'(x) dx, \quad (\text{E.79})$$

$$\tilde{C}_2 = \int (\bar{K}' \star \bar{K}'(z))^2 dz \int (\check{g}_{21}^2(m_2(x))w(m_2(x))m_2'(x))^2 dx \quad (\text{E.80})$$

$$\tilde{E}_3(a^*, b^*) = \int w(t) \check{g}_{11}(t) \check{g}_{21}(t) \int \bar{K}'(z) \bar{K}'(a^* + zb^*) dz dt, \quad (\text{E.81})$$

$$\begin{aligned} \tilde{C}_{3,1}(r) &= \int \int [\int \bar{K}'(x) \bar{K}'(y + r(u)x) dx]^2 [\check{g}_{11}(m_1(u)) \check{g}_{21}(m_1(u)) w(m_1(u)) m_1'(u)]^2 du dy, \\ \tilde{C}_{3,2}(a, b, c) &= \frac{1}{n_1^2 b_{n,1} b_{n,2}^4} \int \int (\check{g}_{11}(m_1(u)) \check{g}_{22}(m_1(u)) w(m_1(u)) m_1'(u))^2 \times \\ &\quad \left[ \int \bar{K}'(x) \bar{K}'(a(u) + b(u)y + c(u)x) dx \int \bar{K}'(y + x) \bar{K}'(a(u) + c(u)x) dx \right] du dy \end{aligned} \quad (\text{E.82})$$

$$\begin{aligned} D_{1,2}(a, b, c) &= \int \int \check{g}_{21}^2(m_1(u)) \check{g}_{11}^2(m_1(u)) [m_1'(u) w(m_1(u))]^2 \left[ \int \bar{K}'(x) \bar{K}'(y + x) dx \right] \\ &\quad \left[ \int \bar{K}'(a(u) + b(u)x) \bar{K}'(a(u) + b(u)x + c(u)y) dx \right] du dy \end{aligned} \quad (\text{E.83})$$

$$\begin{aligned} D_{1,3}(a, b, c) &= \int \int \check{g}_{11}^3(m_1(u)) \check{g}_{21}(m_1(u)) [m_1'(u) w(m_1(u))]^2 \left[ \int \bar{K}'(x) \bar{K}'(y + x) dx \right] \\ &\quad \left[ \int \bar{K}'(x) \bar{K}'(a(u) + b(u)x + c(u)y) dx \right] du dy \end{aligned} \quad (\text{E.84})$$

$$\begin{aligned} D_{2,3}(a, b, c) &= \int \int \check{g}_{21}^3(m_2(u)) \check{g}_{11}(m_2(u)) [m_2'(u) w(m_2(u))]^2 \left[ \int \bar{K}'(x) \bar{K}'(y + x) dx \right] \\ &\quad \left[ \int \bar{K}'(x) \bar{K}'(a(u) + b(u)x + c(u)y) dx \right] du dy \end{aligned} \quad (\text{E.85})$$

Further define for  $a, b, c$  functions of  $u$ ,  $z \in \mathbb{R}$ ,

$$\begin{aligned}
\tilde{I}(z, a, b, c) &= \int \int dudy [w(m_1(u))m_1'(u)]^2 I^2(z, u, a, b, c, y) dudy, \text{ where} \\
I(z, u, a, b, c, y) &= \int \left( z\check{g}_{11}(m_1(u))\bar{K}'(x) - \check{g}_{21}'(m_1(u))\bar{K}'(a(u) + b(u)x) \right) \\
&\quad \times \left( \check{g}_{21}(m_1(u))\bar{K}'(a(u) + b(u)x + c(u)y) - z\check{g}_{12}(m_1(u))\bar{K}'(y + x) \right) dx. \\
\tilde{II}(z, a, b) &= \int \int z^2 \check{g}_{12}^2(m_1(u)) [w(m_1(u))m_1'(u)]^2 II^2(z, u, a, b, c, y) dudy, \text{ where} \\
II(z, u, a, b, y) &= \int \left( z\check{g}_{11}(m_1(u))\bar{K}'(x) - \check{g}_{21}(m_1(u))\bar{K}'(a + bx) \right) \bar{K}'(y + x) dx. \\
\tilde{III}(z, a, b) &= \int \int c_{2,1,n}^2 \check{g}_{11}^2(m_1(u)) [w(m_1(u))m_1'(u)]^2 III^2(z, u, a, b, y) dudy, \text{ where} \\
III(z, u, a, b, y) &= \int \left( -z\check{g}_{12}(m_1(u))\bar{K}'(x) + \check{g}_{22}(m_1(u))\bar{K}'(a + bx) \right) \bar{K}'(y + x) dx. \\
\tilde{IV} &= \int \int [\check{g}_{11}(m_1(u))\check{g}_{12}(m_1(u))w(m_1(u))m_1'(u)]^2 [\bar{K}' \star \bar{K}'(y)]^2 dy du.
\end{aligned}$$

**Theorem E.1** Assume the conditions stated in (A1)-(A6), (A7'), (A8) and (B1), (B2), (B3), and that as  $n \rightarrow \infty$ ,  $n_1/n_2 \rightarrow n_{1,2} \in (0, \infty)$ ,  $b_{n_1}/b_{n_2} \rightarrow b_{1,2} \in (0, \infty)$ ,  $n_{1,2} = 1/n_{2,1}$ ,  $b_{1,2} = 1/b_{2,1}$ ,  $\eta^{-1} = O(\log(n_1 + n_2))$ ,  $\eta = o(1)$ . Further, let  $(m_1^{-1})'(t) - (m_2^{-1})'(t) = \rho_n \kappa(t)$  for some bounded function  $\kappa(t)$ , and  $\rho_n := \rho_{n_1, n_2} = [(n_1 b_{n_1}^{5/2})^{-1/2} (n_2 b_{n_2}^{5/2})^{-1/2}]^{-1/2}$ . Assuming  $\frac{\rho_{n_1, n_2}}{b_{n,1}} = o(1)$ . Let us now define

$$\tilde{B} = n_{2,1} b_{2,1}^{3/2} \tilde{E}_1 + n_{1,2} b_{1,2}^{3/2} \tilde{E}_2 - 2n_{2,1}^{1/2} b_{1,2}^{1/2} \tilde{E}_3(0, b_{1,2}), \quad (\text{E.86})$$

and suppose that the superscript 1-2 mean the exchange of indices 1 and 2. For example, let

$$\tilde{B}^{1-2} = n_{1,2} b_{1,2}^{3/2} \tilde{E}_1^{1-2} + n_{2,1} b_{2,1}^{3/2} \tilde{E}_2^{1-2} - 2n_{1,2}^{1/2} b_{2,1}^{1/2} \tilde{E}_3^{1-2}(0, b_{2,1}), \quad (\text{E.87})$$

where, for instance,

$$\tilde{E}_2^{1-2} = \int \bar{K}'^2(u) du \int \check{g}_{12}^2(m_1(x)) w(m_1(x)) m_1'(x) dx. \quad (\text{E.88})$$

Further, define

$$\begin{aligned}\tilde{V} = & 2\tilde{C}_1 n_{2,1} b_{2,1}^{5/2} + 2\tilde{C}_2 n_{1,2} b_{1,2}^{5/2} + 4n_{2,1} b_{1,2}^{3/2} \tilde{C}_{32}(0, b_{1,2}, b_{1,2}) + 4n_{2,1} b_{1,2}^{3/2} D_{12}(0, b_{1,2}, b_{1,2}) \\ & - 8n_{2,1} b_{2,1}^{1/2} D_{13}(0, b_{1,2}, b_{1,2}) - 8b_{2,1}^{1/2} D_{2,3}(0, b_{2,1}, b_{2,1}),\end{aligned}\quad (\text{E.89})$$

$$\begin{aligned}\tilde{W} = & n_{1,2} b_{1,2}^{11/2} \tilde{I}(n_{2,1} b_{2,1}^2, 0, b_{1,2}, b_{1,2}) - (n_{1,2}^2 - n_{1,2}) b_{1,2}^{11/2} \tilde{I}I(n_{2,1} b_{2,1}^2, 0, b_{1,2}) + (n_{1,2}^2 - \\ & n_{1,2}) b_{1,2}^{11/2} I\tilde{I}I(n_{2,1} b_{2,1}^2, 0, b_{1,2}) - n_{2,1} (1 - n_{2,1})^2 b_{2,1}^{5,2} \tilde{I}\tilde{V}.\end{aligned}\quad (\text{E.90})$$

Now, if  $m_2^{-1}(m_1(0)) = 0$ , we have

$$(n_1 n_2)^{1/2} (b_{n_1}^5 b_{n_2}^5)^{1/4} T_{n_1 n_2} - (b_{n,1} b_{n,2})^{-1/4} (\tilde{B} + \tilde{B}^{1-2}) \Rightarrow N(0, \tilde{V} + \tilde{V}^{1-2} + 4\tilde{W}). \quad (\text{E.91})$$

Now, if  $|m_2^{-1}(m_1(0))| > 0$ , we have

$$(n_1 n_2)^{1/2} (b_{n_1}^5 b_{n_2}^5)^{1/4} T_{n_1 n_2} - (b_{n,1} b_{n,2})^{-1/4} (\underline{\tilde{B}} + \underline{\tilde{B}}^{1-2}) \Rightarrow N(0, \underline{\tilde{V}} + \underline{\tilde{V}}^{1-2} + 4\underline{\tilde{W}}), \quad (\text{E.92})$$

where

$$\begin{aligned}\underline{\tilde{B}} = & n_{2,1} b_{2,1}^{3/2} \tilde{E}_1 + n_{1,2} b_{1,2}^{3/2} \tilde{E}_2, \\ \underline{\tilde{V}} = & 2\tilde{C}_1 n_{2,1} b_{2,1}^{5/2} + 2\tilde{C}_2 n_{1,2} b_{1,2}^{5/2} - 8n_{2,1} b_{2,1}^{1/2} D_{13}(0, b_{1,2}, b_{1,2}) - 8b_{2,1}^{1/2} D_{2,3}(0, b_{2,1}, b_{2,1}),\end{aligned}\quad (\text{E.93})$$

$$\begin{aligned}\underline{\tilde{W}} = & n_{1,2} b_{1,2}^{11/2} \tilde{I}(n_{2,1} b_{2,1}^2, \infty, b_{1,2}, b_{1,2}) - (n_{1,2}^2 - n_{1,2}) b_{1,2}^{11/2} \tilde{I}I(n_{2,1} b_{2,1}^2, \infty, b_{1,2}) + (n_{1,2}^2 - \\ & n_{1,2}) b_{1,2}^{11/2} I\tilde{I}I(n_{2,1} b_{2,1}^2, \infty, b_{1,2}) - n_{2,1} (1 - n_{2,1})^2 b_{2,1}^{5,2} \tilde{I}\tilde{V}.\end{aligned}\quad (\text{E.94})$$

*Proof.* Notice that Propositions 2.1 and D.3 still hold. Therefore, following the proof of Theorem 3.1, we shall see that

$$(n_1 n_2 b_{n,1}^{5/2} b_{n,2}^{5/2})^{1/2} (\tilde{T}_{n_1, n_2} - T_{n_1, n_2}) = o_p(1). \quad (\text{E.95})$$

Here  $\tilde{T}_{n_1, n_2}$  is defined in (B.2), and applying Proposition E.1 instead of Proposition D.1,

we shall see that the decomposition of  $\tilde{T}_{n_1, n_2}$  in (B.10) can be written as

$$\tilde{T}_{n_1, n_2} = \int_{\mathbb{R}} [\rho_n \kappa(t) + Z(t) + R(t)]^2 w(t) dt, \quad (\text{E.96})$$

where  $Z(t)$  is defined in (B.11) replaced by

$$Z(t) = Z_{11}(t) + Z_{12}(t) - Z_{22}(t) - Z_{21}(t). \quad (\text{E.97})$$

Here

$$\begin{aligned} Z_{11}(t) &= \sum_{j=1}^{n_1} W_{11}(j, t) V_{j,1}, \quad W_{11}(j, t) = \sum_{i=1}^N \frac{M_{11}^c(i/N)}{n_1 b_{n,1} N h_1^2} H' \left( \frac{m_1(i/N) - t}{h_1} \right) \bar{K}_{b_{n,1}}(j/n_1 - i/N), \\ Z_{12}(t) &= \sum_{j=1}^{n_1} W_{12}(j, t) V_{j,2}, \quad W_{12}(j, t) = \sum_{i=1}^N \frac{M_{12}^c(i/N)}{n_1 b_{n,1} N h_1^2} H' \left( \frac{m_1(i/N) - t}{h_1} \right) \bar{K}_{b_{n,1}}(j/n_1 - i/N), \\ Z_{21}(t) &= \sum_{j=1}^{n_2} W_{21}(j, t) V_{\lfloor \frac{n_1 j}{n_2} \rfloor, 1}, \quad W_{21}(j, t) = \sum_{i=1}^N \frac{M_{12}^c(i/N)}{n_2 b_{n,2} N h_2^2} H' \left( \frac{m_2(i/N) - t}{h_2} \right) \bar{K}_{b_{n,2}}(j/n_2 - i/N), \\ Z_{22}(t) &= \sum_{j=1}^{n_2} W_{22}(j, t) V_{\lfloor \frac{n_1 j}{n_2} \rfloor, 2}, \quad W_{22}(j, t) = \sum_{i=1}^N \frac{M_{22}^c(i/N)}{n_2 b_{n,2} N h_2^2} H' \left( \frac{m_2(i/N) - t}{h_2} \right) \bar{K}_{b_{n,2}}(j/n_2 - i/N). \end{aligned}$$

For the remaining term  $R(t)$ , it satisfies (B.12). Again following the proof of Theorem 3.1, we shall see that

$$(n_1 n_2 b_{n,1}^{5/2} b_{n,2}^{5/2})^{1/2} \left( \int_{\mathbb{R}} R(t) (R(t) + \rho_n \kappa(t) + Z(t)) w(t) dt + \int_{\mathbb{R}} \rho_n \kappa(t) Z(t) w(t) dt \right) = o_p(1). \quad (\text{E.98})$$

In the following, we shall show that

$$(n_1 b_{n,1}^{5/2} n_2 b_{n,2}^{5/2})^{1/2} \int_{\mathbb{R}} Z^2(t) w(t) dt - (b_{n,1} b_{n,2})^{-1/4} (\tilde{B} + \tilde{B}^{1-2}) \Rightarrow N(0, \tilde{V} + \tilde{V}^{1-2} + 4\tilde{W}) \quad (\text{E.99})$$

for  $m_2^{-1}(m_1(0)) = 0$ , and

$$(n_1 b_{n,1}^{5/2} n_2 b_{n,2}^{5/2})^{1/2} \int_{\mathbb{R}} Z^2(t) w(t) dt - (b_{n,1} b_{n,2})^{-1/4} (\tilde{B} + \tilde{B}^{1-2}) \Rightarrow N(0, \tilde{V} + \tilde{V}^{1-2} + 4\tilde{W}). \quad (\text{E.100})$$

for  $|m_2^{-1}(m_1(0))| > 0$ .

We now calculate the asymptotic variance and bias. To ease the notation, write

$$W(j_1, j_2) = \int W_{11}(j_1, t) W_{11}(j_2, t) w(t) dt, \quad (\text{E.101})$$

$$W'(j_1, j_2) = \int W_{11}(j_1, t) W_{21}(j_2, t) w(t) dt, \quad (\text{E.102})$$

$$W'_{21}(j_1, j_2) = \int W_{21}(j_1, t) W_{21}(j_2, t) w(t) dt. \quad (\text{E.103})$$

Similarly to the proof of Theorem 3.1,  $W_{uv}(j, t)$  can be written as  $\tilde{W}_{uv}(j, t)(1 + O(b_{n,u} + \frac{h_u}{b_{n,u}}))$  for  $u, v = 1, 2$ , where

$$\begin{aligned} \tilde{W}_{uv}(j, t) &= \frac{-1}{n_u b_{n,u}^2} M_{uv}^c(m_u^{-1}(t)) \bar{K}' \left( \frac{j/n_u - m_u^{-1}(t)}{b_{n,u}} \right) ((m_u^{-1})'(t))^2 \int_{\mathbb{R}} H'(y) y dy \\ &= \frac{-1}{n_u b_{n,u}^2} \check{g}_{uv}(t) \bar{K}' \left( \frac{j/n_u - m_u^{-1}(t)}{b_{n,u}} \right), \end{aligned} \quad (\text{E.104})$$

since for notational simplicity we have defined  $M_{12}^c(t) = M_{21}^c(t)$ .

Define  $\tilde{Z}_1(t) = Z_{11}(t) - Z_{21}(t)$  and  $\tilde{Z}_2(t) = Z_{22}(t) - Z_{12}(t)$ , so

$$Z(t) = \tilde{Z}_1(t) - \tilde{Z}_2(t) \quad (\text{E.105})$$

Then

$$\int \tilde{Z}_1^2(t) w(t) dt = \int \left( \sum_{j=1}^{n_1} W_{11}(j, t) V_{j,1} \right)^2 w(t) dt + \int \left( \sum_{j=1}^{n_2} W_{21}(j, t) V_{[n_1 j / n_2], 1} \right)^2 w(t) dt$$

$$-2 \int \sum_{j_1=1}^{n_1} W_{11}(j_1, t) V_{j_1,1} \sum_{j_2=1}^{n_2} W_{21}(j_2, t) V_{\lfloor n_1 j_2 / n_2 \rfloor, 1} w(t) dt := A + B - 2C, \quad (\text{E.106})$$

where  $A$ ,  $B$  and  $C$  are defined in an obvious manner. Following the proof of Theorem 3.1, we shall see that

$$\mathbb{E}(A) = \mathbb{E} \left( \int \left( \sum_{j=1}^{n_1} W_{11}(j, t) V_{j,1} \right)^2 w(t) dt \right) = \frac{1}{n_1 b_{n_1}^3} \tilde{E}_1(1 + o(1)), \quad (\text{E.107})$$

$$\text{Var}(A) = \text{Var} \left( \int \left( \sum_{j=1}^{n_1} W_{11}(j, t) V_{j,1} \right)^2 w(t) dt \right) = \frac{2}{n_1^2 b_{n_1}^5} \tilde{C}_1(1 + o(1)), \quad (\text{E.108})$$

$$\begin{aligned} \mathbb{E}(C) &= \mathbb{E} \left( \int \sum_{j_1=1}^{n_1} W_{11}(j_1, t) V_{j_1,1} \sum_{j_2=1}^{n_2} W_{21}(j_2, t) V_{\lfloor n_1 j_2 / n_2 \rfloor, 1} w(t) dt \right) \\ &= \frac{1}{n_1 b_{n_1} b_{n_2}^2} \tilde{E}_3 \left( \frac{m_1^{-1}(t) - m_2^{-1}(t)}{b_{n,2}}, \frac{b_{n,1}}{b_{n,2}} \right) (1 + o(1)). \end{aligned} \quad (\text{E.109})$$

To calculate  $\text{Var}(C) = \text{Var} \left( \int \sum_{j_1=1}^{n_1} W_{11}(j_1, t) V_{j_1,1} \sum_{j_2=1}^{n_2} W_{21}(j_2, t) V_{\lfloor n_1 j_2 / n_2 \rfloor, 1} w(t) dt \right)$ , notice that

$$\begin{aligned} \text{Var}(C) &= \text{Var} \left( \int \sum_{j_1=1}^{n_1} W_{11}(j_1, t) V_{j_1,1} \sum_{j_2=1}^{n_2} W_{21}(j_2, t) V_{\lfloor n_1 j_2 / n_2 \rfloor, 1} w(t) dt \right) \\ &= \text{Cov} \left( \sum_{j_1=1}^{n_1} \sum_{j_2=1}^{n_2} W'_{21}(j_1, j_2) V_{j_1,1} V_{\lfloor \frac{n_1 j_2}{n_2} \rfloor}, \sum_{j_3=1}^{n_1} \sum_{j_4=1}^{n_2} W'_{21}(j_3, j_4) V_{j_3,1} V_{\lfloor \frac{n_1 j_4}{n_2} \rfloor} \right) \end{aligned} \quad (\text{E.110})$$

When  $j_1 = j_3, j_2 = j_4$  and  $j_1 \neq \lfloor n_1 j / n_2 \rfloor$ , we have

$$\begin{aligned} &\mathbb{E} \sum_{j_1=1}^{n_1} \sum_{j_2=1}^{n_2} \sum_{j_3=1}^{n_1} \sum_{j_4=1}^{n_2} W'_{21}(j_1, j_2) V_{j_1,1} V_{\lfloor \frac{n_1 j_2}{n_2} \rfloor} W'_{21}(j_3, j_4) V_{j_3,1} V_{\lfloor \frac{n_1 j_4}{n_2} \rfloor} \mathbf{1}(j_1 = j_3, j_2 = j_4, j_1 \neq \lfloor \frac{n_1 j_2}{n_2} \rfloor) \\ &= \frac{1}{n_1 b_{n,1}^4 n_2 b_{n,2}^4} \int \int \left[ \int \check{g}_{11}(t) \check{g}_{22}(t) \bar{K}' \left( \frac{u - m_1^{-1}(t)}{b_{n,1}} \right) \bar{K}' \left( \frac{v - m_2^{-1}(t)}{b_{n,2}} \right) w(t) dt \right]^2 dudv (1 + o(1)) \\ &= \frac{1}{n_1 n_2 b_{n,1}^2 b_{n,2}^3} \int \int \left[ \int \bar{K}'(x) \bar{K}'(y + m'_{21}(u) \frac{b_{n,1} x}{b_{n,2}}) dx \right]^2 \\ &\quad \times [\check{g}_{11}(m_1(u)) \check{g}_{21}(m_1(u)) w(m_1(u)) m'_1(u)]^2 dudv (1 + o(1)). \end{aligned} \quad (\text{E.111})$$

Similarly, since

$$W'_{21}(\lfloor \frac{n_1 j_4}{n_2} \rfloor, j_2) = \frac{1}{n_1 n_2 b_{n,1}^2 b_{n,2}^2} \int \check{g}_{11}(t) \check{g}_{21}(t) \bar{K}'(\frac{j_4/n_2 - m_1^{-1}(t)}{b_{n,1}}) \bar{K}'(\frac{j_2/n_2 - m_2^{-1}(t)}{b_{n,2}}) w(t) dt (1 + O(\sum_{s=1}^2 (b_{n,s} + \frac{h_s}{b_{n,s}}))) \quad (\text{E.112})$$

and similarly expression holds for  $W'_{21}(\lfloor \frac{n_1 j_2}{n_2} \rfloor, j_4)$ , we have

$$\begin{aligned} \mathbb{E} \sum_{j_1=1}^{n_1} \sum_{j_2=1}^{n_2} \sum_{j_3=1}^{n_1} \sum_{j_4=1}^{n_2} W'_{21}(j_1, j_2) V_{j_1,1} V_{\lfloor \frac{n_1 j_2}{n_2} \rfloor} W'_{21}(j_3, j_4) V_{j_3,1} V_{\lfloor \frac{n_1 j_4}{n_2} \rfloor} \mathbf{1}(j_1 = \lfloor \frac{n_1 j_4}{n_2} \rfloor, j_3 = \lfloor \frac{n_1 j_2}{n_2} \rfloor, j_1 \neq \lfloor \frac{n_1 j_2}{n_2} \rfloor) \\ = \frac{1}{n_1^2 b_{n,1}^4 b_{n,2}^4} \int \int \left[ \int \check{g}_{11}(t) \check{g}_{22}(t) \bar{K}'(\frac{u - m_1^{-1}(t)}{b_{n,1}}) \bar{K}'(\frac{v - m_2^{-1}(t)}{b_{n,2}}) w(t) dt \right. \\ \left. \times \int \check{g}_{11}(t) \check{g}_{22}(t) \bar{K}'(\frac{v - m_1^{-1}(t)}{b_{n,1}}) \bar{K}'(\frac{u - m_2^{-1}(t)}{b_{n,2}}) w(t) dt \right] dudv (1 + o(1)) \\ = \frac{1}{n_1^2 b_{n,1} b_{n,2}^4} \int \int (\check{g}_{11}(m_1(u)) \check{g}_{22}(m_1(u)) w(m_1(u)) m'_1(u))^2 \\ \times \left[ \int \bar{K}'(x) \bar{K}'(\frac{u - m_{21}(u)}{b_{n,2}} + \frac{b_{n,1}}{b_{n,2}} y + m'_{21}(u) \frac{b_{n,1}}{b_{n,2}} x) dx \right. \\ \left. \times \int \bar{K}'(y + x) \bar{K}'(\frac{u - m_{21}(u)}{b_{n,2}} + m'_{21}(u) \frac{b_{n,1}}{b_{n,2}} x) dx \right] dudv. \end{aligned} \quad (\text{E.113})$$

Also, it can be verified that

$$\begin{aligned} \mathbb{E} \sum_{j_1=1}^{n_1} \sum_{j_2=1}^{n_2} \sum_{j_3=1}^{n_1} \sum_{j_4=1}^{n_2} W'_{21}(j_1, j_2) V_{j_1,1} V_{\lfloor \frac{n_1 j_2}{n_2} \rfloor} W'_{21}(j_3, j_4) V_{j_3,1} V_{\lfloor \frac{n_1 j_4}{n_2} \rfloor} \mathbf{1}(j_1 = \lfloor \frac{n_1 j_4}{n_2} \rfloor, j_3 = \lfloor \frac{n_1 j_2}{n_2} \rfloor = j_1) \\ = o(\frac{1}{n_1^2 b_{n,1}^2 b_{n,2}^3}), \end{aligned} \quad (\text{E.114})$$

Combining (E.111), (E.113) and (E.114), we have

$$\begin{aligned} \text{Var}(C) = \\ (\frac{1}{n_1 n_2 b_{n,1}^2 b_{n,2}^3} \tilde{C}_{3,1}(m'_{21}(u) \frac{b_{n,1}}{b_{n,2}}) + \frac{1}{n_1^2 b_{n,1} b_{n,2}^4} \tilde{C}_{3,2}(\frac{u - m_{21}(u)}{b_{n,2}}, \frac{b_{n,1}}{b_{n,2}}, m'_{21}(u) \frac{b_{n,1}}{b_{n,2}})) (1 + o(1)) \end{aligned} \quad (\text{E.115})$$

Using similar argument, we obtain

$$\begin{aligned}
Cov(A, C) &= Cov\left(\sum_{j_1=1}^{n_1} \sum_{j_2=1}^{n_2} \int W_{11}(j_1, t) W_{11}(j_2, t) w(t) dt V_{j_1,1} V_{j_2,1}, \right. \\
&\quad \left. \sum_{j_3=1}^{n_1} \sum_{j_4=1}^{n_2} \int W_{11}(j_3, t) W_{21}(j_4, t) w(t) dt V_{j_3} V_{\lfloor n_1 j_4 / n_2 \rfloor, 1} \right) \\
&= \frac{2}{n_1^2 b_{n,1}^3 b_{n,2}^2} D_{1,3} \left( \frac{u - m_{21}(u)}{b_{n,2}}, m'_{21}(u) \frac{b_{n,1}}{b_{n,2}}, \frac{b_{n,1}}{b_{n,2}} \right) (1 + o(1))
\end{aligned} \tag{E.116}$$

and

$$Cov(B, C) = \frac{2}{n_1 n_2 b_{n,2}^3 b_{n,1}^2} D_{2,3} \left( \frac{u - m_{12}(u)}{b_{n,1}}, m'_{12}(u) \frac{b_{n,2}}{b_{n,1}}, \frac{b_{n,2}}{b_{n,1}} \right) (1 + o(1)) \tag{E.117}$$

$$Cov(A, B) = \frac{2}{n_1^2 b_{n,1} b_{n,2}^4} D_{1,2} \left( \frac{u - m_{21}(u)}{b_{n,2}}, m'_{21}(u) \frac{b_{n,1}}{b_{n,2}}, \frac{b_{n,1}}{b_{n,2}} \right) (1 + o(1)) \tag{E.118}$$

$$\mathbb{E}(B) = \frac{1}{n_2 b_{n,2}^3} \tilde{E}_2, Var(B) = \frac{2}{n_2^2 b_{n,2}^5} \tilde{C}_2 \tag{E.119}$$

Therefore,

$$\mathbb{E} \int \tilde{Z}_1^2(t) w(t) dt = \left\{ \frac{\tilde{E}_1}{n_1 b_{n,1}^3} + \frac{\tilde{E}_2}{n_2 b_{n,2}^3} - \frac{2}{n_1 b_{n,1} b_{n,2}^2} \tilde{E}_3 \left( \frac{m_1^{-1}(t) - m_2^{-1}(t)}{b_{n,2}}, \frac{b_{n,1}}{b_{n,2}} \right) \right\} (1 + o(1)), \tag{E.120}$$

$$\begin{aligned}
Var \int \tilde{Z}_1^2(t) w(t) dt &= \\
&\left\{ \frac{2\tilde{C}_1}{n_1^2 b_{n,1}^5} + \frac{2\tilde{C}_2}{n_2^2 b_{n,2}^5} + \right. \\
&\left( \frac{4}{n_1 n_2 b_{n,1}^2 b_{n,2}^3} \tilde{C}_{3,1} \left( m'_{21}(u) \frac{b_{n,1}}{b_{n,2}} \right) + \frac{4}{n_1^2 b_{n,1} b_{n,2}^4} \tilde{C}_{3,2} \left( \frac{u - m_{21}(u)}{b_{n,2}}, \frac{b_{n,1}}{b_{n,2}}, m'_{21}(u) \frac{b_{n,1}}{b_{n,2}} \right) \right) \\
&+ \frac{4}{n_1^2 b_{n,1} b_{n,2}^4} D_{1,2} \left( \frac{u - m_{21}(u)}{b_{n,2}}, m'_{21}(u) \frac{b_{n,1}}{b_{n,2}}, \frac{b_{n,1}}{b_{n,2}} \right) - \frac{8}{n_1^2 b_{n,1}^3 b_{n,2}^2} D_{1,3} \left( \frac{u - m_{21}(u)}{b_{n,2}}, m'_{21}(u) \frac{b_{n,1}}{b_{n,2}}, \frac{b_{n,1}}{b_{n,2}} \right) \\
&\left. - \frac{8}{n_1 n_2 b_{n,2}^3 b_{n,1}^2} D_{2,3} \left( \frac{u - m_{12}(u)}{b_{n,1}}, m'_{12}(u) \frac{b_{n,2}}{b_{n,1}}, \frac{b_{n,2}}{b_{n,1}} \right) \right\} (1 + o(1)).
\end{aligned} \tag{E.121}$$

It is easy to see that  $\mathbb{E} \int \tilde{Z}_2^2(t) w(t) dt$  and  $Var \int \tilde{Z}_2^2(t) w(t) dt$  has the same form as that of  $\mathbb{E} \int \tilde{Z}_1^2(t) w(t) dt$  and  $Var \int \tilde{Z}_1^2(t) w(t) dt$  with indices 1 and 2 exchanged. On the other

hand, notice that

$$\int Z^2(t)w(t)dt = \int (\tilde{Z}_1^2(t) + \tilde{Z}_2^2(t) - 2\tilde{Z}_1(t)\tilde{Z}_2(t))w(t)dt.$$

It is obvious that  $\mathbb{E} \int \tilde{Z}_1(t)\tilde{Z}_2(t)w(t)dt = 0$ ,  $Cov(\int \tilde{Z}_1^2(t)w(t)dt, \int \tilde{Z}_2^2(t)w(t)dt) = 0$ ,

$$Cov(\int \tilde{Z}_1^2(t)w(t)dt, \int \tilde{Z}_1(t)\tilde{Z}_2(t)w(t)dt) = 0,$$

and

$$Cov(\int \tilde{Z}_2^2(t)w(t)dt, \int \tilde{Z}_1(t)\tilde{Z}_2(t)w(t)dt) = 0.$$

It remains to calculate  $Var(\int \tilde{Z}_1(t)\tilde{Z}_2(t)w(t)dt)$ . Without loss generality consider  $n_1/n_2 = k \in \mathbb{Z}$  where  $k \geq 1$ . Then, we have

$$\begin{aligned}\tilde{Z}_1(t) &= \sum_{j=1}^{n_1} [W_{11}(j, t) - W_{21}(j/k) \mathbf{1}(j/k \in \mathbb{Z})] V_{j,1} := \sum_{j=1}^{n_1} \tilde{W}_1(j, t) V_{j,1}, \\ \tilde{Z}_2(t) &= \sum_{j_1=1}^{n_1} [W_{22}(j/k, t) \mathbf{1}(j/k \in \mathbb{Z}) - W_{12}(j, t)] V_{j,2} := \sum_{j=1}^{n_1} \tilde{W}_2(j, t) V_{j,2},\end{aligned}$$

where  $\tilde{W}_1(j, t)$  and  $\tilde{W}_2(j, t)$  are defined in an obvious way. Further, define

$$\tilde{W}_{11}(j, t) = W_{11}(j, t) - W_{21}(j/k, t), \quad (\text{E.122})$$

$$\tilde{W}_{22}(j, t) = W_{22}(j/k, t) - W_{12}(j, t). \quad (\text{E.123})$$

Let us now define

$$V = \int \tilde{Z}_1(t)\tilde{Z}_2(t)w(t)dt = \sum_{j_1=1}^{n_1} \sum_{j_2=1}^{n_1} \int \tilde{W}_1(j_1, t)\tilde{W}_2(j_2, t)w(t)dt V_{j_1,1} V_{j_2,1}. \quad (\text{E.124})$$

Hence,

$$Var(V) = \sum_{j_1=1}^{n_1} \sum_{j_2=1}^{n_1} \left[ \int \tilde{W}_1(j_1, t)\tilde{W}_2(j_2, t)w(t)dt \right]^2$$

$$\begin{aligned}
&= \sum_{j_1=1}^{n_1} \sum_{j_2=1}^{n_1} \left[ \int (\tilde{W}_{11}(j_1, t) \mathbf{1}(j_1/k \in \mathbb{Z}) + W_{11}(j_1, t) \mathbf{1}(j_1/k \notin \mathbb{Z})) \right. \\
&\quad \left. (\tilde{W}_{22}(j_2, t) \mathbf{1}(j_2/k \in \mathbb{Z}) - W_{12}(j_2, t) \mathbf{1}(j_1/k \notin \mathbb{Z})) w(t) dt \right]^2 \\
&:= I - II + III - IV,
\end{aligned}$$

where

$$I = \sum_{j_1=1}^{n_1} \sum_{j_2=1}^{n_1} \left[ \int \tilde{W}_{11}(j_1, t) \tilde{W}_{22}(j_2, t) \mathbf{1}(j_1/k \in \mathbb{Z}) \mathbf{1}(j_2/k \in \mathbb{Z}) w(t) dt \right]^2, \quad (\text{E.125})$$

$$II = \sum_{j_1=1}^{n_1} \sum_{j_2=1}^{n_1} \left[ \int \tilde{W}_{11}(j_1, t) W_{12}(j_2, t) \mathbf{1}(j_1/k \in \mathbb{Z}) \mathbf{1}(j_2/k \notin \mathbb{Z}) w(t) dt \right]^2, \quad (\text{E.126})$$

$$III = \sum_{j_1=1}^{n_1} \sum_{j_2=1}^{n_1} \left[ \int W_{11}(j_1, t) \tilde{W}_{22}(j_2, t) \mathbf{1}(j_1/k \notin \mathbb{Z}) \mathbf{1}(j_2/k \in \mathbb{Z}) w(t) dt \right]^2, \quad (\text{E.127})$$

$$IV = \sum_{j_1=1}^{n_1} \sum_{j_2=1}^{n_1} \left[ \int W_{11}(j_1, t) W_{12}(j_2, t) \mathbf{1}(j_1/k \notin \mathbb{Z}) \mathbf{1}(j_2/k \notin \mathbb{Z}) w(t) dt \right]^2. \quad (\text{E.128})$$

To sake of notational complexity, write  $c_{2,1,n} = \frac{n_2 b_{n,2}^2}{n_1 b_{n,1}^2}$ ,  $m_{12}(u) = (m_1)^{-1}(m_2(u))$ . Then via tedious calculus, we see that

$$I = \frac{b_{n,1}^3}{n_2^2 b_{n,2}^8} \tilde{I}(c_{2,1,n}, \frac{u - m_{21}(u)}{b_{n,2}}, \frac{b_{n,1}}{b_{n,2}} m'_{21}(u), \frac{b_{n,1}}{b_{n,2}}) (1 + o(1))$$

For  $II$ , by Riemann sum approximation, we see that

$$\begin{aligned}
II = \frac{(k-1)n_1^2}{k^2(n_2 b_{n,2}^2)^4} \int \int \left\{ c_{2,1,n} \check{g}_{11}(t) \bar{K}'\left(\frac{u - m_1^{-1}(t)}{b_{n,1}}\right) - \check{g}_{21}(t) \bar{K}'\left(\frac{u - m_2^{-1}(t)}{b_{n,2}}\right) \right. \\
\left. \times c_{2,1,n} \check{g}_{12}(t) \bar{K}'\left(\frac{v - m_1^{-1}(t)}{b_{n,1}}\right) w(t) dt \right\}^2 dudv (1 + o(1)),
\end{aligned}$$

and therefore,

$$II = \frac{(n_1 - n_2) b_{n,1}^3}{n_2^3 b_{n,2}^8} \tilde{II}(c_{2,1,n}, \frac{u - m_{21}(u)}{b_{n,2}}, \frac{b_{n,1}}{b_{n,2}} m'_{21}(u)) (1 + o(1))$$

Using the same argument, we have

$$III = \frac{(n_1 - n_2)b_{n,1}^3}{n_2^3 b_{n,2}^8} \tilde{I} \tilde{I} I(c_{2,1,n}, \frac{u - m_{21}(u)}{b_{n,2}}, \frac{b_{n,1}}{b_{n,2}} m'_{21}(u))(1 + o(1))$$

Finally,

$$IV = \left( \frac{n_1 - n_2}{n_1} \right)^2 \frac{1}{n_1^2 b_{n,1}^5} \tilde{I} \tilde{V} (1 + o(1))$$

In summary,  $Var(V)$  equals with

$$\begin{aligned} &= \left\{ \frac{b_{n,1}^3}{n_2^3 b_{n,2}^8} \tilde{I}(c_{2,1,n}, \frac{u - m_{21}(u)}{b_{n,2}}, \frac{b_{n,1}}{b_{n,2}} m'_{21}(u), \frac{b_{n,1}}{b_{n,2}}) - \frac{(n_1 - n_2)b_{n,1}^3}{n_2^3 b_{n,2}^8} \tilde{I} \tilde{I}(c_{2,1,n}, \frac{u - m_{21}(u)}{b_{n,2}}, \frac{b_{n,1}}{b_{n,2}} m'_{21}(u)) \right. \\ &+ \left. \frac{(n_1 - n_2)b_{n,1}^3}{n_2^3 b_{n,2}^8} \tilde{I} \tilde{I} I(c_{2,1,n}, \frac{u - m_{21}(u)}{b_{n,2}}, \frac{b_{n,1}}{b_{n,2}} m'_{21}(u)) - \left( \frac{n_1 - n_2}{n_1} \right)^2 \frac{1}{n_1^2 b_{n,1}^5} \tilde{I} \tilde{V} \right\} (1 + o(1)) \end{aligned} \quad (\text{E.129})$$

Therefore, the asymptotic bias and variance of (E.99) and (E.100) follow from (E.120),(E.121), the term obtained by (E.120),(E.121) via swapping indices 1 and 2, (E.129) and Proposition E.2. The asymptotic normality follows tedious calculation via Theorem 2.1 of de Jong (1987) and the independence of centered  $\int \tilde{Z}_1^2(t)w(t)dt$ ,  $\int \tilde{Z}_2^2(t)w(t)dt$  and  $\int \tilde{Z}_1(t)\tilde{Z}_2(t)w(t)dt$ . Therefore, (E.99) and (E.100) hold and the proof of theorem follows.  $\square$

**Theorem E.2** Assume the conditions stated in (A1)-(A6), (A7'), (A8) and (B1), (B2), (B3), and suppose that as  $n \rightarrow \infty$ ,  $n_1/n_2 \rightarrow n_{1,2} \in (0, \infty)$ ,  $b_{n,1}/b_{n,2} \rightarrow b_{1,2} \in (0, \infty)$ ,  $h_2/h_1 \rightarrow h_{1,2} \in (0, \infty)$ ,  $n_{1,2} = 1/n_{2,1}$ ,  $b_{1,2} = 1/b_{2,1}$ ,  $h_{1,2} = 1/h_{2,1}$ ,  $\eta^{-1} = O(\log(n_1 + n_2))$ ,  $\eta = o(1)$ . For  $u = 1, 2$  and  $v = 1, 2$ , let

$$\check{g}_{uv}^\circ(t) = M_{uv}^c(m_u^{-1}(t))((m_u^{-1})'(t)) \int_{\mathbb{R}} H''(y) y dy. \quad (\text{E.130})$$

Define

$$\bar{K}_1^\circ(t) = \left( (n_{2,1} b_{2,1}^3)^{1/2} \check{g}_{11}^{\circ^2}(t) + (n_{1,2} b_{1,2})^{1/2} \check{g}_{21}^{\circ^2}(t) \right)^2 \int \bar{K}'^2(x) dx$$

$$-2\check{g}_{11}^{\circ^2}(t)\check{g}_{21}^{\circ^2}(t)n_{2,1}^{1/2}b_{1,2}^{1/2} \int \bar{K}'(x)\bar{K}'(b_{1,2}x)dx \mathbf{1}(m_{21}(0) = 0), \quad (\text{E.131})$$

$$\begin{aligned} \bar{K}_2^\circ(t) &= \left( (n_{2,1}b_{2,1}h_{2,1}^4)^{1/2}\check{g}_{11}^{\circ^2}(t) + (n_{1,2}b_{1,2}h_{1,2}^4)^{1/2}\check{g}_{21}^{\circ^2}(t) \right)^2 \int \bar{K}^2(x)dx \\ &\quad - 2\check{g}_{11}^{\circ^2}(t)\check{g}_{21}^{\circ^2}(t)n_{2,1}^{1/2}b_{1,2}^{1/2} \int \bar{K}(x)\bar{K}(b_{1,2}x)dx \mathbf{1}(m_{21}(0) = 0), \end{aligned} \quad (\text{E.132})$$

and consequently,

$$K_1^\circ(t) = \bar{K}_1^\circ(t) + (\bar{K}_1^\circ)^{1-2}(t), \quad (\text{E.133})$$

$$K_2^\circ(t) = \bar{K}_2^\circ(t) + (\bar{K}_2^\circ)^{1-2}(t). \quad (\text{E.134})$$

Now, if  $(m_1^{-1})'(t) - (m_2^{-1})'(t) = \rho_{n_1, n_2} \kappa(t)$  for some non-zero bounded function  $\kappa(t)$  and  $\rho_{n_1, n_2} = o(\eta \wedge b_{n,1})$ , then as  $\min(n_1, n_2) \rightarrow \infty$ , we have

$$\mathbb{P} \left( \sup_{t \in \mathcal{I}_{\hat{a}, \hat{b}}} \frac{(n_1 b_{n,1}^3 n_2 b_{n,2}^3)^{1/4} |(\hat{m}_1^{-1})'(t) - (\hat{m}_2^{-1})'(t) - ((m_1^{-1})'(t) - (m_2^{-1})'(t))|}{K_1^{\circ^{1/2}}(t)} \geq \sqrt{-2 \log(\pi \alpha / \kappa_0)} \right) \rightarrow \alpha, \quad (\text{E.135})$$

where  $\mathcal{I}_{\hat{a}, \hat{b}} = (\hat{a} + \eta, \hat{b} - \eta)$  and

$$\kappa_0 = \frac{(b_{n,1}b_{n,2})^{1/2}}{h_1 h_2} \int_{m_1(0)}^{m_1(1-m_2^{-1}(m_1(0)))} \left( \frac{K_2(t)}{K_1(t)} \right)^{1/2} dt. \quad (\text{E.136})$$

*Proof.* Without loss of generality, consider  $n_1 \geq n_2$  and that  $n_1/n_2 = k$  for some integer  $k$ . Following the proof of Theorem 3.2, it suffices to evaluate  $\mathbb{E}(Z^2(t))$ ,  $\mathbb{E}(Z'^2(t))$  and  $\mathbb{E}(Z(t)Z'(t))$ , where now  $Z(t)$  is defined in (E.97). Once the above quantities are obtained, the theorem will follow from an application of Proposition 1 of Sun and Loader (1994) and the same argument as given in the proof of Theorem 3.2.

Recall the decomposition of  $Z(t)$  in (E.105).

$$\mathbb{E}Z^2(t) = \mathbb{E}\tilde{Z}_1^2(t) + \mathbb{E}\tilde{Z}_2^2(t), \quad (\text{E.137})$$

and recall the definition of  $W_{uv}(j, t)$ ,  $u, v \in \{1, 2\}^2$  in the proof of Theorem E.62.

$$\begin{aligned}\mathbb{E}\tilde{Z}_1^2(t) &= \sum_{j=1}^{n_1} [W_{11}^2(j, t) - W_{21}(j/k, t)\mathbf{1}(j/k \in \mathbb{Z})]^2 \\ &= \sum_{j=1}^{n_1} W_{11}(j, t) + \sum_{j=1}^{n_1} W_{21}^2(j/k, t)\mathbf{1}(j/k \in \mathbb{Z}) - 2 \sum_{j=1}^{n_1} W_{11}(j, t)W_{21}(j/k, t)\mathbf{1}(j/k \in \mathbb{Z}).\end{aligned}\tag{E.138}$$

By the similar but simpler argument than the proof of Theorem E.1, we have

$$\sum_{j=1}^{n_1} W_{11}^2(j, t) = \frac{1}{n_1 b_{n,1}^3} \check{g}_{11}^2(t) \int \bar{K}'^2(x) dx (1 + o(1)), \tag{E.139}$$

$$\sum_{j=1}^{n_1} W_{21}^2(j/k, t)\mathbf{1}(j/k \in \mathbb{Z}) = \frac{1}{n_2 b_{n,2}^3} \check{g}_{21}^2(t) \int \bar{K}'^2(x) dx (1 + o(1)), \tag{E.140}$$

$$\begin{aligned}\sum_{j=1}^{n_1} W_{11}(j, t)W_{21}(j/k, t)\mathbf{1}(j/k \in \mathbb{Z}) &= \frac{\check{g}_{11}(t)\check{g}_{21}(t)}{n_1 b_{n,1} b_{n,2}^2} \int \bar{K}'(x) \\ &\quad \times \bar{K}'\left(\frac{m_1^{-1}(t) - m_2^{-1}(t) + x b_{n,1}}{b_{n,2}}\right) dx (1 + o(1)).\end{aligned}\tag{E.141}$$

Therefore,

$$\begin{aligned}\mathbb{E}(\tilde{Z}_1^2(t)) &= \left( \frac{1}{n_1 b_{n,1}^3} \check{g}_{11}^2(t) \int \bar{K}'^2(x) dx + \frac{1}{n_2 b_{n,2}^3} \check{g}_{21}^2(t) \int \bar{K}'^2(x) dx \right. \\ &\quad \left. - 2 \frac{\check{g}_{11}(t)\check{g}_{21}(t)}{n_1 b_{n,1} b_{n,2}^2} \int \bar{K}'(x) \bar{K}'\left(\frac{m_1^{-1}(t) - m_2^{-1}(t) + x b_{n,1}}{b_{n,2}}\right) dx \right) (1 + o(1)),\end{aligned}\tag{E.142}$$

$$\mathbb{E}(\tilde{Z}_2^2(t)) = (\mathbb{E}(\tilde{Z}_1^2(t)))^{1-2}. \tag{E.143}$$

To calculate  $\mathbb{E}(Z'(t)) = \mathbb{E}(\tilde{Z}_1'^2(t)) + \mathbb{E}(\tilde{Z}_2'^2(t))$ , similarly to the proof of Theorem 3.1,  $\frac{\partial}{\partial t} W_{uv}(j, t)$  can be written as  $\tilde{W}'_{uv}(j, t)(1 + o(1))$  for  $u, v = 1, 2$ , where

$$\begin{aligned}\tilde{W}'_{uv}(j, t) &= \frac{-1}{n_u b_{n,u} h_u^2} M_{uv}^c(m_u^{-1}(t)) \bar{K} \left( \frac{j/n_u - m_u^{-1}(t)}{b_{n,u}} \right) ((m_u^{-1})'(t)) \int_{\mathbb{R}} H''(y) y dy \\ &:= \frac{-1}{n_u b_{n,u} h_u^2} \check{g}_{uv}^\circ(t) \bar{K} \left( \frac{j/n_u - m_u^{-1}(t)}{b_{n,u}} \right).\end{aligned}\tag{E.144}$$

Here  $\check{g}_{uv}^\circ(t)$  is defined in a straightforward way. Using this fact, it follows that

$$\sum_{j=1}^{n_1} W_{11}'^2(j, t) = \frac{(\check{g}_{11}^\circ(t))^2}{n_1 b_{n,1} h_1^4} \int \bar{K}^2(x) dx (1 + o(1)), \quad (\text{E.145})$$

$$\sum_{j=1}^{n_1} W_{21}'^2(j/k, t) \mathbf{1}(j/k \in \mathbb{Z}) = \frac{(\check{g}_{21}^\circ(t))^2}{n_2 b_{n,2} h_2^4} \int \bar{K}^2(x) dx (1 + o(1)), \quad (\text{E.146})$$

$$\begin{aligned} \sum_{j=1}^{n_1} W_{11}'(j, t) W_{21}'(j/k, t) \mathbf{1}(j/k \in \mathbb{Z}) &= \frac{\check{g}_{11}^\circ(t) \check{g}_{21}^\circ(t)}{n_1 b_{n,2} h_1^2 h_2^2} \int \bar{K}(x) \\ &\times \bar{K}\left(\frac{m_1^{-1}(t) - m_2^{-1}(t) + x b_{n,1}}{b_{n,2}}\right) dx (1 + o(1)). \end{aligned} \quad (\text{E.147})$$

Hence

$$\begin{aligned} \mathbb{E}(\tilde{Z}_1'^2(t)) &= \left( \frac{(\check{g}_{11}^\circ(t))^2}{n_1 b_{n,1} h_1^4} \int \bar{K}^2(x) dx + \frac{(\check{g}_{21}^\circ(t))^2}{n_2 b_{n,2} h_2^4} \int \bar{K}^2(x) dx \right. \\ &\quad \left. - 2 \frac{\check{g}_{11}^\circ(t) \check{g}_{21}^\circ(t)}{n_1 b_{n,2} h_1^2 h_2^2} \int \bar{K}(x) \bar{K}\left(\frac{m_1^{-1}(t) - m_2^{-1}(t) + x b_{n,1}}{b_{n,2}}\right) dx \right), \end{aligned} \quad (\text{E.148})$$

$$\mathbb{E}(\tilde{Z}_2'^2(t)) = (\mathbb{E}(\tilde{Z}_1'^2(t)))^{1-2} \quad (\text{E.149})$$

Following the proof of Theorem 3.2, we have

$$\mathbb{E}(\tilde{Z}(t) \tilde{Z}'(t)) = O\left(\frac{1}{n_1 b_{n,1}^2 h_1^2} \frac{h_1}{b_{n,1}}\right) = o\left(\frac{1}{n_1 b_{n,1}^2 h_1^2}\right). \quad (\text{E.150})$$

Therefore, the theorem follows from (E.142), (E.143), (E.148), (E.149), (E.150) and Proposition E.2.  $\square$

**Proof of Theorem 5.1.** The theorem directly follows from the proof of Theorem E.1 and Theorem E.2. Notice that under the null hypothesis, the asymptotic results of Theorem E.1 and Theorem E.2 will differ between the scenarios of  $d = m_{21}(0) = 0$  and  $d = m_{21}(0) \neq 0$ .  $\square$

## F Results of Simulation Study : Dependent Data

In Section 5.2 in the main manuscript, we briefly discuss the results of simulation studies for dependent data sets. The detailed results are reported here. The results in Tables 1, 2, 3 and 4 indicate that the estimated sizes of the SIT test and the SCB test (described in Section 5 in the main article) are not deviated more than 1% from the estimated sizes when the data sets are independent, and the estimated powers of the SIT test and the SCB test are not deviated more than 6% from the estimated powers when the data sets are independent.

| model                                                                | $n = 100$             | $n = 500$             |
|----------------------------------------------------------------------|-----------------------|-----------------------|
| Example 1 ( $\alpha = 5\%$ , $\tau = 0.5$ , $b_{n,s} = n_s^{-1/4}$ ) | (0.061, 0.058, 0.063) | (0.050, 0.055, 0.049) |
| Example 1 ( $\alpha = 5\%$ , $\tau = 0.5$ , $b_{n,s} = n_s^{-1/5}$ ) | (0.055, 0.058, 0.059) | (0.052, 0.054, 0.050) |
| Example 1 ( $\alpha = 5\%$ , $\tau = 0.7$ , $b_{n,s} = n_s^{-1/4}$ ) | (0.056, 0.061, 0.060) | (0.052, 0.051, 0.055) |
| Example 1 ( $\alpha = 5\%$ , $\tau = 0.7$ , $b_{n,s} = n_s^{-1/5}$ ) | (0.057, 0.062, 0.060) | (0.051, 0.053, 0.052) |
| Example 1 ( $\alpha = 5\%$ , $\tau = 0.8$ , $b_{n,s} = n_s^{-1/4}$ ) | (0.053, 0.052, 0.058) | (0.055, 0.052, 0.051) |
| Example 1 ( $\alpha = 5\%$ , $\tau = 0.8$ , $b_{n,s} = n_s^{-1/5}$ ) | (0.055, 0.056, 0.052) | (0.053, 0.051, 0.051) |
| Example 2 ( $\alpha = 5\%$ , $\tau = 0.5$ , $b_{n,s} = n_s^{-1/4}$ ) | (0.057, 0.058, 0.055) | (0.050, 0.053, 0.056) |
| Example 2 ( $\alpha = 5\%$ , $\tau = 0.5$ , $b_{n,s} = n_s^{-1/4}$ ) | (0.051, 0.055, 0.054) | (0.052, 0.054, 0.050) |
| Example 2 ( $\alpha = 5\%$ , $\tau = 0.7$ , $b_{n,s} = n_s^{-1/4}$ ) | (0.054, 0.055, 0.058) | (0.052, 0.054, 0.050) |
| Example 2 ( $\alpha = 5\%$ , $\tau = 0.7$ , $b_{n,s} = n_s^{-1/5}$ ) | (0.053, 0.061, 0.059) | (0.054, 0.049, 0.051) |
| Example 2 ( $\alpha = 5\%$ , $\tau = 0.8$ , $b_{n,s} = n_s^{-1/4}$ ) | (0.053, 0.062, 0.058) | (0.054, 0.050, 0.052) |
| Example 2 ( $\alpha = 5\%$ , $\tau = 0.8$ , $b_{n,s} = n_s^{-1/5}$ ) | (0.051, 0.056, 0.056) | (0.052, 0.050, 0.050) |

Table 1: *The estimated size of the SIT test for different sample sizes  $n_1 = n_2 = n$ . The levels of significance (denoted as  $\alpha$ ) is 5% for dependent data. In each cell, from the left, the first, the second and the third values are corresponding to  $w_{n,s} = n_s^{-1/3}$ ,  $n_s^{-1/5}$  and  $n_s^{-1/7}$ , respectively.*

## References

de Jong, P. (1987). A central limit theorem for generalized quadratic forms. *Probability Theory and Related Fields*, 75(2):261–277.

| model                                                                | $n = 100$             | $n = 500$             |
|----------------------------------------------------------------------|-----------------------|-----------------------|
| Example 1 ( $\alpha = 5\%$ , $\tau = 0.5$ , $b_{n,s} = n_s^{-1/4}$ ) | (0.062, 0.055, 0.064) | (0.053, 0.054, 0.051) |
| Example 1 ( $\alpha = 5\%$ , $\tau = 0.5$ , $b_{n,s} = n_s^{-1/5}$ ) | (0.062, 0.059, 0.062) | (0.053, 0.051, 0.050) |
| Example 1 ( $\alpha = 5\%$ , $\tau = 0.7$ , $b_{n,s} = n_s^{-1/4}$ ) | (0.063, 0.061, 0.064) | (0.052, 0.050, 0.055) |
| Example 1 ( $\alpha = 5\%$ , $\tau = 0.7$ , $b_{n,s} = n_s^{-1/5}$ ) | (0.052, 0.061, 0.063) | (0.050, 0.053, 0.055) |
| Example 1 ( $\alpha = 5\%$ , $\tau = 0.8$ , $b_{n,s} = n_s^{-1/4}$ ) | (0.057, 0.056, 0.058) | (0.051, 0.050, 0.051) |
| Example 1 ( $\alpha = 5\%$ , $\tau = 0.8$ , $b_{n,s} = n_s^{-1/5}$ ) | (0.058, 0.055, 0.054) | (0.056, 0.055, 0.055) |
| Example 2 ( $\alpha = 5\%$ , $\tau = 0.5$ , $b_{n,s} = n_s^{-1/4}$ ) | (0.050, 0.056, 0.054) | (0.050, 0.051, 0.054) |
| Example 2 ( $\alpha = 5\%$ , $\tau = 0.5$ , $b_{n,s} = n_s^{-1/4}$ ) | (0.052, 0.055, 0.057) | (0.050, 0.052, 0.056) |
| Example 2 ( $\alpha = 5\%$ , $\tau = 0.7$ , $b_{n,s} = n_s^{-1/4}$ ) | (0.057, 0.059, 0.059) | (0.054, 0.056, 0.054) |
| Example 2 ( $\alpha = 5\%$ , $\tau = 0.7$ , $b_{n,s} = n_s^{-1/5}$ ) | (0.055, 0.057, 0.058) | (0.056, 0.052, 0.054) |
| Example 2 ( $\alpha = 5\%$ , $\tau = 0.8$ , $b_{n,s} = n_s^{-1/4}$ ) | (0.055, 0.062, 0.059) | (0.055, 0.052, 0.058) |
| Example 2 ( $\alpha = 5\%$ , $\tau = 0.8$ , $b_{n,s} = n_s^{-1/5}$ ) | (0.055, 0.058, 0.060) | (0.052, 0.055, 0.059) |

Table 2: *The estimated size of the SCB test for different sample sizes  $n_1 = n_2 = n$  for dependent data. The levels of significance (denoted as  $\alpha$ ) are 5% and 10%. In each cell, from the left, the first, the second and the third values are corresponding to  $w_{n,s} = n_s^{-1/3}$ ,  $n_s^{-1/5}$  and  $n_s^{-1/7}$ , respectively.*

- Dette, H., Dhar, S. S., and Wu, W. (2021). Identifying shifts between two regression curves. *Annals of the Institute of Statistical Mathematics*, 73:855–889.
- Dette, H., Neumeyer, N., and Pilz, K. F. (2006). A simple nonparametric estimator of a strictly monotone regression function. *Bernoulli*, 12(3):469–490.
- Dette, H. and Wu, W. (2019). Detecting relevant changes in the mean of nonstationary processes—a mass excess approach. *The Annals of Statistics*, 47(6):3578–3608.
- Sun, J. and Loader, C. R. (1994). Simultaneous confidence bands for linear regression and smoothing. *The Annals of Statistics*, 22(3):1328–1345.
- Wu, W. and Zhou, Z. (2017). Nonparametric inference for time-varying coefficient quantile regression. *Journal of Business & Economic Statistics*, 35(1):98–109.
- Zhou, Z. and Wu, W. B. (2010). Simultaneous inference of linear models with time varying coefficients. *Journal of the Royal Statistical Society: Series B (Statistical Methodology)*, 72(4):513–531.

| model                                                                | $n = 100$             | $n = 500$             |
|----------------------------------------------------------------------|-----------------------|-----------------------|
| Example 3 ( $\alpha = 5\%$ , $\tau = 0.5$ , $b_{n,s} = n_s^{-1/4}$ ) | (0.477, 0.454, 0.491) | (0.749, 0.777, 0.763) |
| Example 3 ( $\alpha = 5\%$ , $\tau = 0.5$ , $b_{n,s} = n_s^{-1/5}$ ) | (0.461, 0.475, 0.502) | (0.781, 0.799, 0.795) |
| Example 3 ( $\alpha = 5\%$ , $\tau = 0.7$ , $b_{n,s} = n_s^{-1/4}$ ) | (0.505, 0.517, 0.522) | (0.774, 0.841, 0.833) |
| Example 3 ( $\alpha = 5\%$ , $\tau = 0.7$ , $b_{n,s} = n_s^{-1/5}$ ) | (0.479, 0.581, 0.543) | (0.865, 0.803, 0.888) |
| Example 3 ( $\alpha = 5\%$ , $\tau = 0.8$ , $b_{n,s} = n_s^{-1/4}$ ) | (0.475, 0.496, 0.517) | (0.872, 0.831, 0.900) |
| Example 3 ( $\alpha = 5\%$ , $\tau = 0.8$ , $b_{n,s} = n_s^{-1/5}$ ) | (0.534, 0.540, 0.522) | (0.888, 0.849, 0.903) |
| Example 4 ( $\alpha = 5\%$ , $\tau = 0.5$ , $b_{n,s} = n_s^{-1/4}$ ) | (0.477, 0.486, 0.532) | (0.817, 0.833, 0.825) |
| Example 4 ( $\alpha = 5\%$ , $\tau = 0.5$ , $b_{n,s} = n_s^{-1/5}$ ) | (0.512, 0.471, 0.510) | (0.833, 0.855, 0.895) |
| Example 4 ( $\alpha = 5\%$ , $\tau = 0.7$ , $b_{n,s} = n_s^{-1/4}$ ) | (0.534, 0.555, 0.527) | (0.870, 0.879, 0.904) |
| Example 4 ( $\alpha = 5\%$ , $\tau = 0.7$ , $b_{n,s} = n_s^{-1/5}$ ) | (0.543, 0.555, 0.565) | (0.875, 0.899, 0.909) |
| Example 4 ( $\alpha = 5\%$ , $\tau = 0.8$ , $b_{n,s} = n_s^{-1/4}$ ) | (0.471, 0.492, 0.505) | (0.843, 0.868, 0.881) |
| Example 4 ( $\alpha = 5\%$ , $\tau = 0.8$ , $b_{n,s} = n_s^{-1/5}$ ) | (0.468, 0.471, 0.499) | (0.902, 0.908, 0.922) |

Table 3: *The estimated power of the SIT test for different sample sizes  $n_1 = n_2 = n$  for dependent data. The levels of significance (denoted as  $\alpha$ ) is 5%. In each cell, from the left, the first, the second and the third values are corresponding to  $w_{n,s} = n_s^{-1/3}$ ,  $n_s^{-1/5}$  and  $n_s^{-1/7}$ , respectively.*

| model                                                                | $n = 100$             | $n = 500$             |
|----------------------------------------------------------------------|-----------------------|-----------------------|
| Example 3 ( $\alpha = 5\%$ , $\tau = 0.5$ , $b_{n,s} = n_s^{-1/4}$ ) | (0.471, 0.425, 0.475) | (0.722, 0.757, 0.743) |
| Example 3 ( $\alpha = 5\%$ , $\tau = 0.5$ , $b_{n,s} = n_s^{-1/5}$ ) | (0.444, 0.468, 0.498) | (0.743, 0.788, 0.802) |
| Example 3 ( $\alpha = 5\%$ , $\tau = 0.7$ , $b_{n,s} = n_s^{-1/4}$ ) | (0.484, 0.488, 0.491) | (0.786, 0.822, 0.813) |
| Example 3 ( $\alpha = 5\%$ , $\tau = 0.7$ , $b_{n,s} = n_s^{-1/5}$ ) | (0.511, 0.527, 0.535) | (0.903, 0.841, 0.865) |
| Example 3 ( $\alpha = 5\%$ , $\tau = 0.8$ , $b_{n,s} = n_s^{-1/4}$ ) | (0.489, 0.472, 0.511) | (0.844, 0.845, 0.890) |
| Example 3 ( $\alpha = 5\%$ , $\tau = 0.8$ , $b_{n,s} = n_s^{-1/5}$ ) | (0.496, 0.502, 0.498) | (0.855, 0.872, 0.894) |
| Example 4 ( $\alpha = 5\%$ , $\tau = 0.5$ , $b_{n,s} = n_s^{-1/4}$ ) | (0.492, 0.475, 0.557) | (0.842, 0.859, 0.871) |
| Example 4 ( $\alpha = 5\%$ , $\tau = 0.5$ , $b_{n,s} = n_s^{-1/5}$ ) | (0.500, 0.484, 0.499) | (0.844, 0.866, 0.884) |
| Example 4 ( $\alpha = 5\%$ , $\tau = 0.7$ , $b_{n,s} = n_s^{-1/4}$ ) | (0.498, 0.506, 0.525) | (0.845, 0.872, 0.877) |
| Example 4 ( $\alpha = 5\%$ , $\tau = 0.7$ , $b_{n,s} = n_s^{-1/5}$ ) | (0.504, 0.528, 0.544) | (0.848, 0.866, 0.887) |
| Example 4 ( $\alpha = 5\%$ , $\tau = 0.8$ , $b_{n,s} = n_s^{-1/4}$ ) | (0.442, 0.459, 0.472) | (0.810, 0.835, 0.844) |
| Example 4 ( $\alpha = 5\%$ , $\tau = 0.8$ , $b_{n,s} = n_s^{-1/5}$ ) | (0.455, 0.468, 0.479) | (0.829, 0.856, 0.883) |

Table 4: *The estimated power of the SCB test for different sample sizes  $n_1 = n_2 = n$  for dependent data. The levels of significance (denoted as  $\alpha$ ) is 5%. In each cell, from the left, the first, the second and the third values are corresponding to  $w_{n,s} = n_s^{-1/3}$ ,  $n_s^{-1/5}$  and  $n_s^{-1/7}$ , respectively.*
